# Supplementary material for: Distribution-Free Conformal Joint Prediction Regions for Neural Marked Temporal Point Processes
Source: arXiv:2401.04612 source file (2024-06-05)
Supplement: Supplementary file 1 [file oldappendix.tex]

\section{Old Results}

\begin{figure}
    \centering
    \includegraphics[width=\linewidth]{images/real_world_metrics/per_model/CLNM_old.pdf}
    \caption{Performance of all methods on real world datasets using the CLNM model. Non-conformal methods are hatched. As expected, all conformal methods achieve marginal coverage. All conformal methods also achieve a relatively good conditional coverage. The size of the prediction region is indicated relative to the smallest run for each dataset and model. C-HDR achieves the smallest prediction region size except for LastFM and Retweets.}
\end{figure}

\begin{figure}
    \centering
    \includegraphics[width=\linewidth]{images/real_world_metrics/per_model/RMTPP_old.pdf}
    \caption{Performance of all methods on real world datasets using the RMTPP model. Non-conformal methods are hatched. As expected, all conformal methods achieve marginal coverage. All conformal methods also achieve a relatively good conditional coverage. The size of the prediction region is indicated relative to the smallest run for each dataset and model. C-HDR achieves the smallest prediction region size except for LastFM and Retweets.}
\end{figure}

\begin{figure}
    \centering
    \includegraphics[width=\linewidth]{images/real_world_metrics/per_model/FNN_old.pdf}
    \caption{Performance of all methods on real world datasets using the FNN model. Non-conformal methods are hatched. As expected, all conformal methods achieve marginal coverage. All conformal methods also achieve a relatively good conditional coverage. The size of the prediction region is indicated relative to the smallest run for each dataset and model. C-HDR achieves the smallest prediction region size except for LastFM and Retweets.}
\end{figure}

\begin{figure}
    \centering
    \includegraphics[width=\linewidth]{images/real_world_metrics/per_model/THP_old.pdf}
    \caption{Performance of all methods on real world datasets using the THP model. Non-conformal methods are hatched. As expected, all conformal methods achieve marginal coverage. All conformal methods also achieve a relatively good conditional coverage. The size of the prediction region is indicated relative to the smallest run for each dataset and model. C-HDR achieves the smallest prediction region size except for LastFM and Retweets.}
\end{figure}

\begin{figure}
    \centering
    \includegraphics[width=\linewidth]{images/real_world_metrics/per_model/SAHP_old.pdf}
    \caption{Performance of all methods on real world datasets using the SAHP model. Non-conformal methods are hatched. As expected, all conformal methods achieve marginal coverage. All conformal methods also achieve a relatively good conditional coverage. The size of the prediction region is indicated relative to the smallest run for each dataset and model. C-HDR achieves the smallest prediction region size except for LastFM and Retweets.}
\end{figure}

\section{Conformal prediction}

\paragraph{Split-conformal prediction}

Conformal prediction is a technique that transforms any heuristic notion of uncertainty generated by any model into a rigorous one.

\begin{enumerate}
\item Split data into two non-overlapping parts, $\mc{D}_{\text{train}} \cup \mc{D}_{\text{cal}} = \mc{D}$

\item Train your model on $\mc{D}_{\text{train}}$ and define a heuristic notion of uncertainty.
\item Define the (non-conformity) score function $s(x,y) \in \mathbb{R}$ which assign larger scores to worse agreement between $x$ and $y$.
\item Compute the scores $S_i = s(X_i,Y_i)$ using $\mc{D}_{\text{cal}}$.
\item Compute $\hat{q} = \text{Quantile}(1 - \alpha; \Set{S_i}_{i=1}^{|\mc{D}_{\text{cal}}|} \cup \Set{\infty})$
\item Use $\hat{q}$ to form the prediction sets for new examples:
\[
\hat{R}(X_{n+1}) = \{y: s(X_{n+1}, y) \leq \hat{q}\} 
\]
\end{enumerate}

\paragraph{Quantile Lemma}

If $S_1, \dots, S_n, S_{n+1}$ are exchangeable random variables, then for any miscoverage $\alpha \in (0, 1)$, we have
\[
\mathbb{P}\left\{ S_{n+1} \leq \text{Quantile}\left(1 - \alpha; \{S_i\}_{i=1}^n \cup \{\infty\}\right) \right\}  \geq 1 - \alpha.
\]

If ties between $S_1, \dots, S_n, S_{n+1}$ occur with probability zero, then the above probability is upper bound by $1 - \alpha + \frac{1}{n+1}$.
In the following, we present Conformalized Quantile Regression (CQR) \cite{Romano2019-kp} and Adaptive Prediction Sets (APS) \cite{Romano2020-ed} for regression and classification, respectively. 

\paragraph{Conformalized Quantile Regression}

CQR is based on the following nonconformity score:
\[
s_\text{CQR}(x, y) = \max\Set{ \hat{Q}_{Y \mid X=x}(\nicefrac{\alpha}{2}) - y, y - \hat{Q}_{Y \mid X=x}(1 - \nicefrac{\alpha}{2})}.
\]

The conformal procedure is:
\begin{enumerate}
    \item Use $\hat{Q}_{Y \mid X}(\alpha/2)$ and $\hat{Q}_{Y \mid X}(1 - \alpha/2)$ trained on $\mc{D}_{\text{train}}$ as heuristic notion of uncertainty
    \item Compute $S_i = s_\text{CQR}(X_i, Y_i)$ for $(X_i, Y_i) \in \mc{D}_{\text{cal}}$
    \item Let $\hat{q} = \text{Quantile}(1 - \alpha; \Set{S_i}_{i=1}^{|\mc{D}_{\text{cal}}|} \cup \Set{\infty})$
    \item Compute 
    \[
    \hat{R}(X_{n+1}) = [\hat{Q}_{Y \mid X=X_{n+1}}(\nicefrac{\alpha}{2}) - \hat{q}, \hat{Q}_{Y \mid X=X_{n+1} }(1 - \nicefrac{\alpha}{2}) + \hat{q}].
    \]
\end{enumerate}

We can write 
\begin{align*}
    &Y_{n+1} \in \hat{R}(X_{n+1}) \iff s_\text{CQR}(X_{n+1}, Y_{n+1}) \leq \hat{q}
\end{align*}

The finite-sample coverage is obtained using the quantile lemma:
\begin{align*}
    \mb{P}(Y_{n+1} \in \hat{R}(X_{n+1})
    &= \mb{P}(s_\text{CQR}(X_{n+1}, Y_{n+1}) \leq \hat{q}) \geq 1 - \alpha.
\end{align*}

\paragraph{Split Conformal classification with Adaptive Prediction Sets}

APS is based on the following nonconformity score:
\begin{center}
    $s_\text{APS}(x, y) = \sum_{y' : \hat{p}(x)_{y'} \geq \hat{p}(x)_{y}} \hat{p}(x)_{y'}$,
\end{center}
where $\hat{p}(x) \in \Delta(|\mathbb{K}|)$, and $\hat{p}(x)_y$ is the probability assigned to class $y \in \mathbb{K}$.

\begin{enumerate}
    \item Use $\hat{p}(\cdot)$ trained on $\mc{D}_{\text{train}}$ as heuristic notion of uncertainty
    \item Compute $S_i = s_\text{APS}(X_i, Y_i)$ for $(X_i, Y_i) \in \mc{D}_{\text{cal}}$
    \item Let $\hat{q} = \text{Quantile}(1 - \alpha; \Set{S_i}_{i=1}^{|\mc{D}_{\text{cal}}|} \cup \Set{\infty})$
    \item Define $\hat{R}(X_{n+1})$ as follows:
    \begin{enumerate}
        \item Let $\pi(X_{n+1})$ be a permutation of $\{1, \dots, K\}$ that sorts the entries of $\hat{p}(X_{n+1})$ in decreasing order.
        \item Define $k = \sup \left\{ k' : \sum_{j=1}^{k'} \hat{p}(X_{n+1})_{\pi_j(X_{n+1})} \leq \hat{q} \right\}$ 
        \item $\hat{R}(X_{n+1}) = \{ \pi_1(X_{n+1}), \dots, \pi_k(X_{n+1}) \}$
    \end{enumerate}
\end{enumerate}

We can show that
\[
Y_{n+1} \in \hat{R}(X_{n+1}) \iff s_\text{APS}(X_{n+1}, Y_{n+1}) \leq \hat{q}.
\]

\begin{itemize}
    \item The conformal guarantee holds for \textbf{arbitrarily bad} base models. 
    \begin{itemize}
    \item    If scores correctly rank errors, easy inputs yield smaller sets, hard inputs yield larger sets.
    \item If scores are bad (like random noise), the sets contain random labels  but will be large enough to provide the conformal guarantee.
    \end{itemize}

    \item While the conformal guarantee always holds, \textbf{better score functions} will provide more \textbf{informative} prediction sets.
\end{itemize}

\section{(Old stuff) Conformalized Neural MTPP}

Let $\mathcal{S} = \{\mathcal{S}_i\}_{i=1}^n$ be a set of $n$ \textbf{exchangeable} sequences where $\mathcal{S}_i = \{e_j \}_{j = 1}^{m_i}$. Following \cite{Stankeviciute2021-ay}, we build input-output pairs as follows 
\[
\mathcal{D} = \left\{\left(e_{1:m_i-1}^{(i)}, e_{m_i}^{(i)} \right)  = \left(X_i, Y_i \right) \right\}_{i = 1}^n,
\]
where $e_{1:m_i-1}^{(i)} = [e_1^{(i)}, \dots, e_{m_i - 1}^{(i)}]$ and $e_{m_i}^{(i)} = (\tau_{m_i}^{(i)}, k_{m_i}^{(i)})$.

Using the standard approaches, we can produce prediction regions \textbf{individually} for the time and mark.

CQR produces prediction regions $\hat{R}_\tau(X_{n+1}) \subseteq \mathbb{R}^+$ such that:
\begin{equation}
    \mathbb{P}(\tau_{m_{n+1}}^{(n+1)} \in \hat{R}_\tau(X_{n+1})) \geq 1 - \alpha.
\end{equation}
APS produces prediction regions $\hat{R}_k(X_{n+1}) \subseteq \mathbb{K}$ such that:
\begin{equation}
    \mathbb{P}(k_{m_{n+1}}^{(n+1)} \in \hat{R}_k(X_{n+1})) \geq 1 - \alpha.
\end{equation}

\paragraph{Joint prediction regions}

Instead of predicting regions for the individual variables, we want a \textbf{joint} prediction region $\hat{R}_{\tau, k}(X_{n+1}) \subseteq \mathbb{K} \times \mathbb{R}^+$ such that:
\begin{equation}
    \mathbb{P}(Y_{n+1} \in \hat{R}_{\tau, k}(X_{n+1})) \geq 1 - \alpha.
\end{equation}

A naive approach is to \textbf{combine independent prediction regions} $\hat{R}_k(X_{n+1})$ and $\hat R_\tau(X_{n+1})$ with nominal level $1 - \nicefrac{\alpha}{2}$.

By the union bound, $\hat R_{k, \tau}(X_{n+1}) = \hat{R}_k(X_{n+1}) \times \hat R_\tau(X_{n+1})$ has coverage at least $1 - \alpha$:
\begin{align}
    &\mathbb{P}(Y_{n+1} \in \hat{R}_k(X_{n+1}) \times \hat R_\tau(X_{n+1})) \\
    =& \mathbb{P}(\tau_{l_{n+1}}^{n+1} \in \hat{R}_k(X_{n+1}) \wedge k_{l_{n+1}}^{n+1} \in \hat R_\tau(X_{n+1})) \\
    =& 1 - \underbrace{\mathbb{P}(\tau_{l_{n+1}}^{n+1} \not\in \hat{R}_k(X_{n+1}) \vee k_{l_{n+1}}^{n+1} \not\in \hat R_\tau(X_{n+1}))}_{\leq \nicefrac{\alpha}{2} + \nicefrac{\alpha}{2}} \\ 
    %=& 1 - \underbrace{\mathbb{P}(\tau_{l_{n+1}}^{n+1} \not\in \hat{R}_k(X_{n+1}))}_{\leq \frac{\alpha}{2}} - \underbrace{\mathbb{P}(k_{l_{n+1}}^{n+1} \not\in \hat R_\tau(X_{n+1}))}_{\leq \frac{\alpha}{2}} \\
    %&+ \underbrace{\mathbb{P}(Y_{n+1} \not\in \hat{R}_k(X_{n+1}) \times \hat R_\tau(X_{n+1}))}_{\geq 0} \\
    \geq& 1 - \alpha
\end{align}

However, the naive approach can be over-conservative with poor statistical efficiency.

\paragraph{Highest Density Regions}

A better approach would take the dependence between the mark and time into account, encouraging the model to exclude unlikely combinations of the two from the predicted region.

Highest Density Regions (HDR, \citet*{Hyndman1996-wx}) for $f(y \mid X=x)$ can be defined as the regions with highest density, namely:
%  will select the points $y$ that are above a minimum density level $z_{1 - \alpha}$
\begin{gather*}
    \text{HDR}(1 - \alpha \mid x) = \Set{y \mid f(y \mid x) \geq z_{1 - \alpha}} \text{ where} \\
    z_{1 - \alpha} \text{ is the largest value satisfying } \mathbb{P}(f(Y \mid x) \geq z_{1 - \alpha}) \geq 1 - \alpha.
\end{gather*}

$\text{HDR}(1 - \alpha \mid x)$ are the smallest regions with coverage $1 - \alpha$.

\begin{figure}
    \centering
    \includegraphics[width=\linewidth]{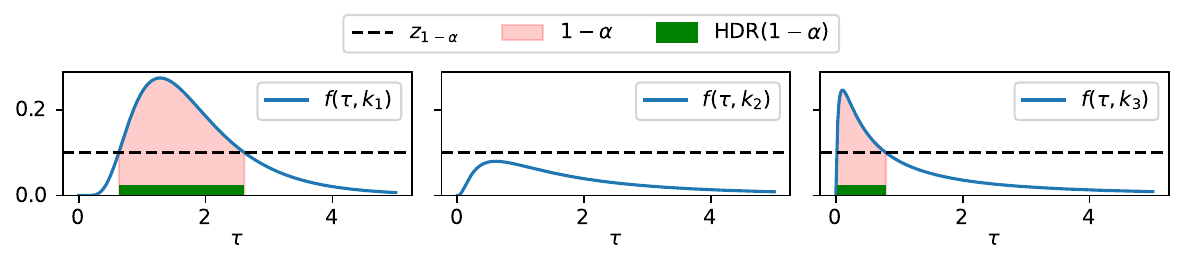}
    \caption{Example of Highest Density Region on a joint density for the inter-arrival time and the mark with three possible labels $k_1$, $k_2$ and $k_3$.}
\end{figure}

\paragraph{HPD-Split}

Building on \citet*{Izbicki2022-ru},  we want to generate conformal prediction regions based on HDRs, called HPD-Split.
The nonconformity score of HPD-Split is:
\begin{gather*}
    s_\text{HPD}(x, y) = \text{HPD}(y \mid x) = \int_{\Set{y' \mid \hat{f}(y' \mid x) \geq \hat{f}(y \mid x)}} \hat{f}(y' \mid x) dy'.
\end{gather*}

\begin{enumerate}
    \item Use $\hat{f}(\cdot|x)$ trained on $\mc{D}_{\text{train}}$ as heuristic notion of uncertainty
    \item Compute HPD scores $S_i = s_\text{HPD}(X_i, Y_i)$ for $(X_i, Y_i) \in \mc{D}_{\text{cal}}$
    \item Let $\hat{q} = \text{Quantile}(1 - \alpha; \Set{S_i}_{i=1}^{|\mc{D}_{\text{cal}}|} \cup \Set{\infty})$
    \item Define $\hat{R}(X_{n+1}) = \text{HDR}(\hat{q} \mid X_{n+1})$
\end{enumerate}

We can show that $Y_{n+1} \in \hat{R}(X_{n+1}) \iff s_\text{HPD}(X_{n+1}, Y_{n+1}) \leq \hat{q}$.

By definition\footnote{To simplify notations, we remove the dependence on $x$.}, we have
\[
\text{HDR}(\hat{q}) = \Set{y \mid \hat{f}(y) \geq z_{\hat{q}}}, 
\]
where
\begin{align*}
	z_{\hat{q}} &= \sup\Set{z' \mid \mathbb{P}(\hat{f}(Y) \geq z') \geq \hat{q}}
	= \sup\Set{z' \mid 1 - \hat{q} \geq F_Z(z')}
	= F_Z^{-1}(1 - \hat{q}),
\end{align*}
and $Z = \hat{f}(Y)$. 

This implies that
\begin{align*}
\text{HDR}(\hat{q}) &= \Set{y \mid \hat{f}(y) \geq z_{\hat{q}}} = \Set{y \mid \hat{f}(y) \geq F_Z^{-1}(1 - \hat{q})} = \Set{y \mid F_Z(\hat{f}(y)) \geq 1 - \hat{q}}.
\end{align*}
and
\begin{align*}
Y_{n+1} \in \text{HDR}(\hat{q})
\iff F_Z(\hat{f}(Y_{n+1})) \geq 1 - \hat{q}
&\iff \hat{q} \geq 1 - F_Z(\hat{f}(Y_{n+1})) \\
&\iff \text{HPD}(Y_{n+1}) \leq \hat{q},
\end{align*}
where
\begin{align*}
\text{HPD}(y) &= \int_{\Set{y' \mid \hat{f}(y') \geq \hat{f}(y)}} \hat{f}(y') dy' = \mathbb{P}(Z \geq \hat{f}(y)) = 1 - F_Z(\hat{f}(y)).
\end{align*}

\section{Miscellaneous}

\bmhead{Quantile function} The quantile function $F^{\ast -1}(\alpha)$ can be expressed in terms of the inverse cumulative intensity function:
\begin{align}
    &F^\ast(\tau) = \alpha \\
    &\iff 1 - \text{exp}(-\Lambda^\ast(t_{i-1} + \tau) = \alpha \\
    &\iff \Lambda^\ast(t_{i-1} + \tau) = - \text{log }(1-\alpha) \\
    &\iff \tau = \Lambda^{\ast-1}\left(-\text{log }(1 - \alpha)\right)- t_{i-1}
\end{align}
\begin{equation}
    F^{\ast-1}(\alpha) = \Lambda^{\ast-1}\left(-\text{log }(1 - \alpha)\right)- t_{i-1}
    \label{eq:inverse_cumul}
\end{equation}

\dobox{ Specific TPP conformal scores?s (lambda, cum lambda, Triangular maps? Random change point theorem, equiv. Distributional conformal)}
\dobox{Compute HDR for the indepnedent case (does it simplify in terms of lambda)? - the naive case}

\bmhead{HDP-split in terms of the conditional intensity}

Note: This requires to change to a notation conditional to $\boldsymbol{h}_{n+1}$.

We can express the conformity score of HDP-split in terms of the intensity as:
\begin{align*}
    s_\text{HPD}((\tau,k)) &= \sum \int_{\Set{(\tau',k') \mid \hat{f}^\ast(\tau',k') \geq \hat{f}^\ast(\tau,k)}} \hat{f}^\ast(\tau', k') d\tau' \\
    &= \sum \int_{\Set{(t',k') \mid \hat{\lambda}_{k'}^\ast(t')\text{exp}\left(-\sum_{k'=1}^K \hat{\Lambda}_{k'}^\ast(t')\right) \geq \hat{\lambda}_{k}^\ast(t)\text{exp}\left(-\sum_{k=1}^K \hat{\Lambda}_k^\ast(t)\right)}} \hat{\lambda}_{k'}^\ast(t')\text{exp}\left(-\sum_{k'=1}^K \hat{\Lambda}_{k'}^\ast(t')\right) dt' \\
    &= 1 - F_Z\left(\hat{\lambda}_{k}^\ast(t)\text{exp}\left(-\sum_{k=1}^K \hat{\Lambda}_k^\ast(t)\right)\right).
\end{align*}
where $Z = \hat{\lambda}_{k'}^\ast(t')\text{exp}\left(-\sum_{k'=1}^K \hat{\Lambda}_{k'}^\ast(t')\right)$.

\section{Experiments}

\bmhead{Observations}
\begin{itemize}
    \item The region lengths for C-HDR are very large on LastFM. Why ? Same remark for C-Naive on Reddit. 
    \item For C-HDR on LastFM, $\hat{q} \simeq 0.99$, which explains the large average region lengths of    . See Figure \ref{fig:scores}.  
\end{itemize}

\begin{table}[h!]
\setlength\tabcolsep{1.5pt}
\centering
\caption{Average coverage and length of the prediction regions generated by the Naive, Naive-C, HDR and C-HDR methods for various models and datasets.}
\begin{tabular}{ccccccccccccc}
\toprule
& && \multicolumn{4}{c}{Coverage} &&& \multicolumn{4}{c}{Length} \\
& && Naive & C-Naive & HDR &   C-HDR &&& Naive &    C-Naive & HDR &      C-HDR \\
\midrule
\multirow{ 6}{*}{CLNM} 
        &LastFM &&                     0.425 &       0.846 &               0.425 &     0.818 &  &&                  0.739 &       9.838 &                    0.38 &    36.489 \\
          &MOOC &  &                   0.637 &       0.818 &                   0.711 &     0.805 &&&                     0.652 &       1.736 &                   0.068 &     0.267 \\
        &Github & &                    0.568 &       0.842 &                   0.621 &     0.905 &&&                     2.305 &       7.405 &                   1.641 &     7.239 \\
        &Reddit &  &                   0.322 &       0.811 &                   0.694 &     0.819 & &&                    3.668 &      27.764 &                   2.463 &     5.873 \\
      &Retweets &   &                  0.408 &       0.801 &                   0.503 &      0.79 &  &&                   1.516 &       6.124 &                   1.817 &     6.435 \\
&Stack O. &     &                0.633 &       0.834 &                   0.699 &     0.827 &     &    &            1.048 &        2.12 &                   1.008 &     1.656 \\
\midrule
\multirow{ 6}{*}{THP}
         &LastFM &   &                  0.513 &       0.844 &                   0.487 &     0.722 && &                    1.077 &      11.403 &                   0.927 &     4.679 \\
           &MOOC &    &                 0.799 &        0.82 &                  0.678 &     0.643 & &  &                  0.328 &       1.149 &                   0.292 &     0.201 \\
         &Github &     &                0.453 &       0.863 &                  0.484 &       0.6 &  &  &                  0.76 &       9.666 &                   0.754 &     3.395 \\
         &Reddit &      &                0.13 &       0.812 &                   0.315 &     0.482 &  &  &                 0.174 &      24.361 &                   0.159 &      1.54 \\
       &Retweets &       &              0.349 &       0.804 &                  0.463 &     0.762 &    &  &               0.867 &       6.583 &                   1.297 &     5.728 \\
 &Stack O. &     &                0.399 &        0.82 &                   0.416 &     0.787 &  &    &               0.414 &       1.991 &                   0.395 &     2.255 \\
\midrule
\multirow{ 6}{*}{FNN}
&LastFM &  &                   0.584 &       0.784 &                   0.697 &     0.754 & &&                    65.61 &      17.174 &                   56.82 &   125.818 \\
&MOOC &   &                   0.37 &       0.841 &                   0.793 &     0.922 &  &&                 229.533 &       9.675 &                 199.981 &   486.425 \\
&Github &   &                  0.768 &       0.884 &                   0.821 &     0.884 & &&                    5.582 &      21.291 &                   5.022 &     8.891 \\
&Reddit &    &                 0.724 &       0.851 &                   0.862 &     0.799 &   &&                187.945 &      62.076 &                  149.99 &   142.457 \\
&Retweets &&                     0.467 &       0.867 &                   0.918 &     0.762 & &&                  13.783 &       7.389 &                  20.647 &     5.629 \\
&Stack O. &   &                  0.712 &       0.826 &                   0.815 &     0.809 & &&                   33.661 &       5.255 &                  26.191 &    25.017 \\
\bottomrule
\end{tabular}
\end{table}

\begin{figure}[h!]
    \centering
    \includegraphics[width=\textwidth]{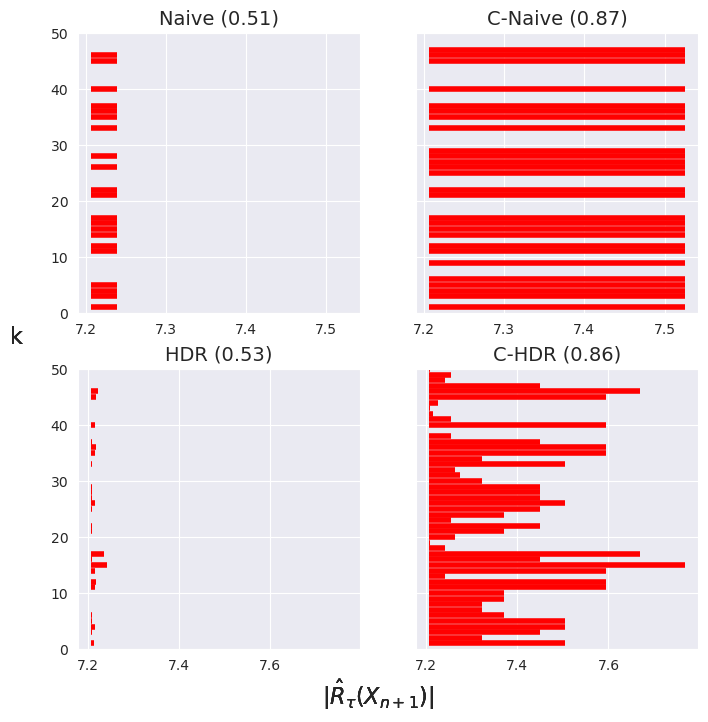}
    \caption{Average length of the prediction regions generated by the Naive, Naive-C, HDR, and C-HDR methods on a test sequence of the LastFM dataset. The miscoverage level is set to $\alpha=0.2$.}
    \label{fig:intervals}
\end{figure}

\begin{figure}[ht!]
        \centering
        \begin{subfigure}[b]{0.49\textwidth}
        \includegraphics[width=\textwidth]{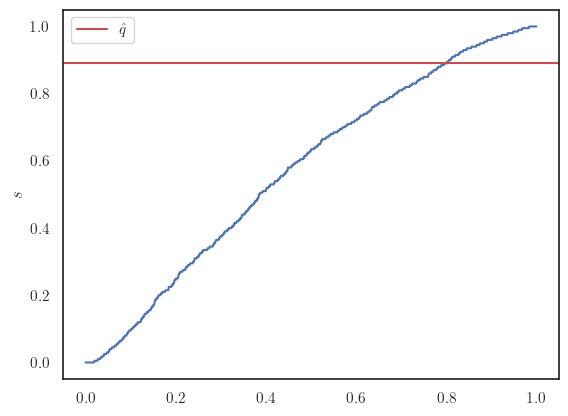}
    \end{subfigure}
    \begin{subfigure}[b]{0.49\textwidth}
        \includegraphics[width=\textwidth]{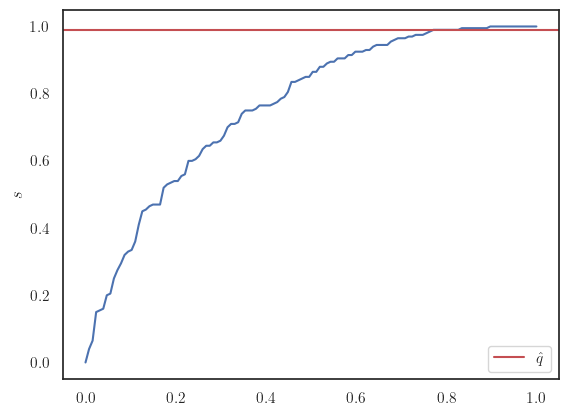}
    \end{subfigure}
    \caption{Distribution of the C-HDR scores for MOOC (left) and LastFM (right). For MOOC, $\hat{q} = 0.89$, and for LastFM, $\hat{q} = 0.99$.}
    \label{fig:scores}
\end{figure}

\begin{figure}[ht!]
        \centering
    \begin{subfigure}[b]{0.32\textwidth}
        \includegraphics[width=\textwidth]{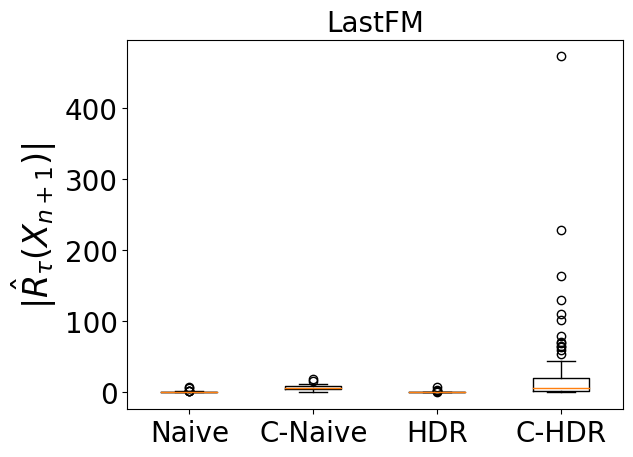}
    \end{subfigure}
    \begin{subfigure}[b]{0.32\textwidth}
        \includegraphics[width=\textwidth]{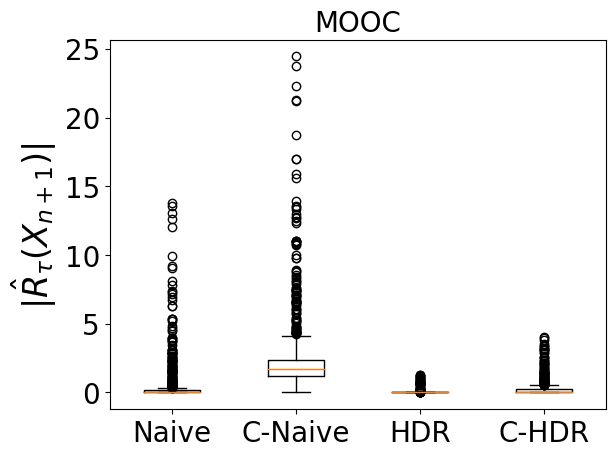}
    \end{subfigure}
    \begin{subfigure}[b]{0.32\textwidth}
        \includegraphics[width=\textwidth]{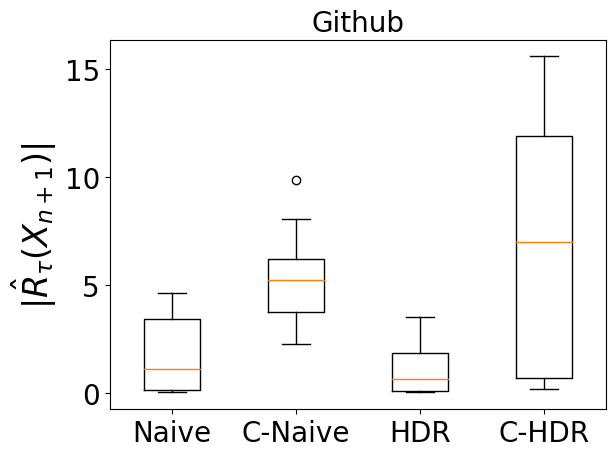}
    \end{subfigure}

    \begin{subfigure}[b]{0.32\textwidth}
        \includegraphics[width=\textwidth]{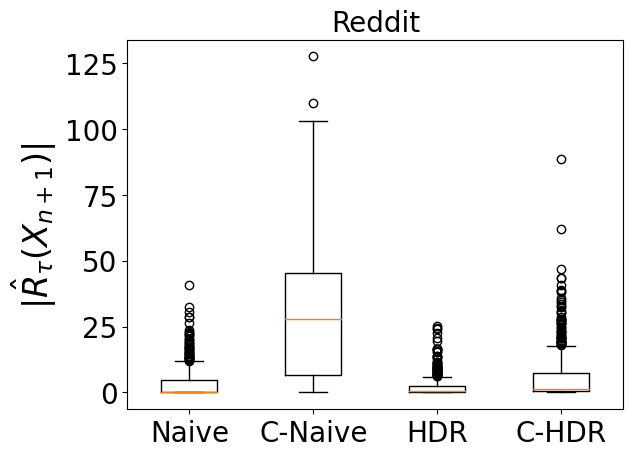}
    \end{subfigure}
    \begin{subfigure}[b]{0.32\textwidth}
        \includegraphics[width=\textwidth]{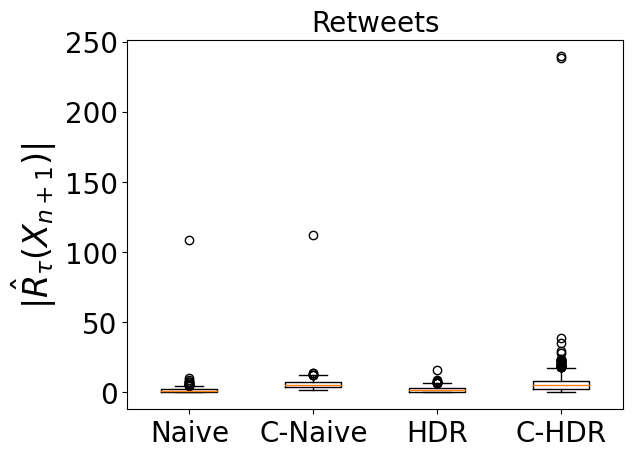}
    \end{subfigure}
    \begin{subfigure}[b]{0.32\textwidth}
        \includegraphics[width=\textwidth]{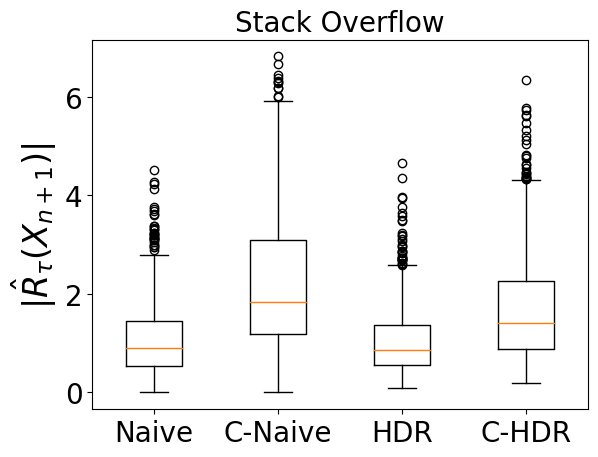}
    \end{subfigure}
    
    \caption{Boxplots of the region lengths generated by the Naive, C-Naive, HDR and C-HDR methods for CLNM on all datasets. Pay attention to the magnitude of the y-axis.}
    \label{fig:dis_lengths}
\end{figure}

\begin{figure}[ht!]
        \centering
    \begin{subfigure}[b]{0.49\textwidth}
        \includegraphics[width=\textwidth]{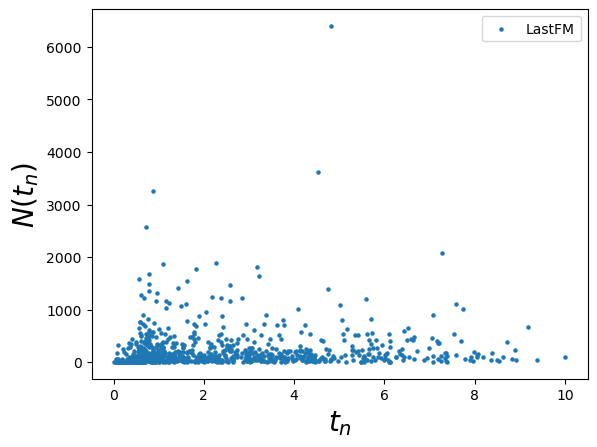}
    \end{subfigure}
    \begin{subfigure}[b]{0.49\textwidth}
        \includegraphics[width=\textwidth]{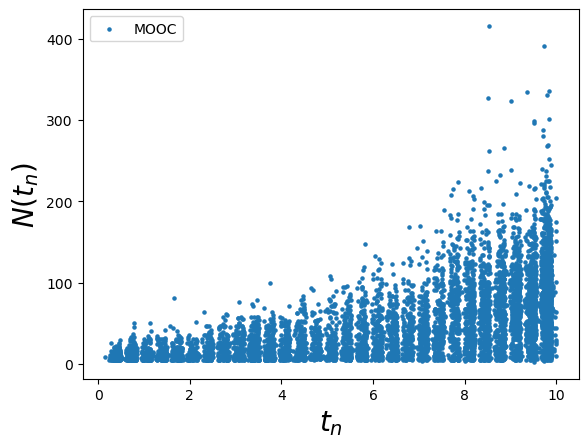}
    \end{subfigure}
    
    \begin{subfigure}[b]{0.49\textwidth}
        \includegraphics[width=\textwidth]{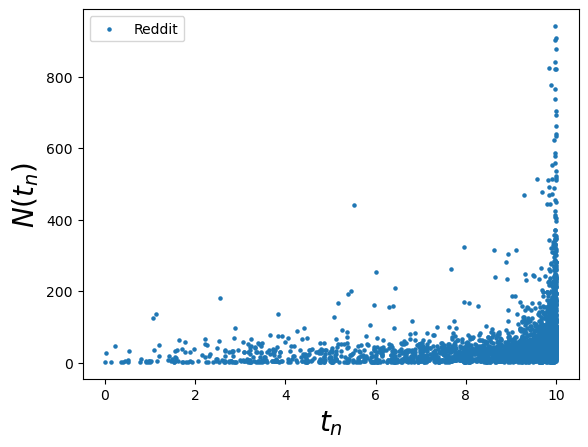}
    \end{subfigure}
    \begin{subfigure}[b]{0.49\textwidth}
        \includegraphics[width=\textwidth]{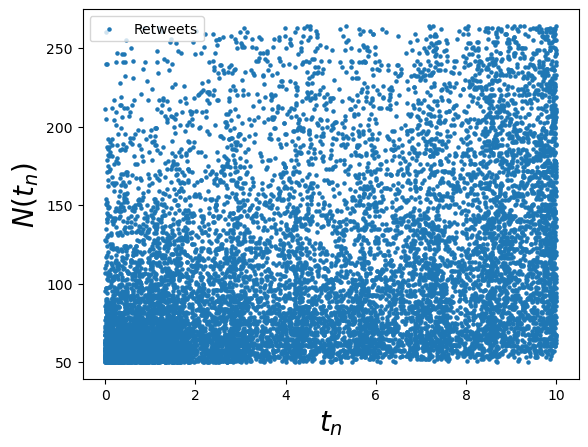}
    \end{subfigure}

    \begin{subfigure}[b]{0.49\textwidth}
        \includegraphics[width=\textwidth]{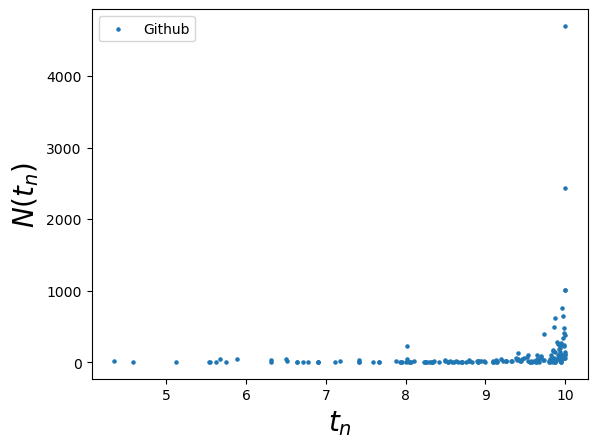}
    \end{subfigure}
    \begin{subfigure}[b]{0.49\textwidth}
        \includegraphics[width=\textwidth]{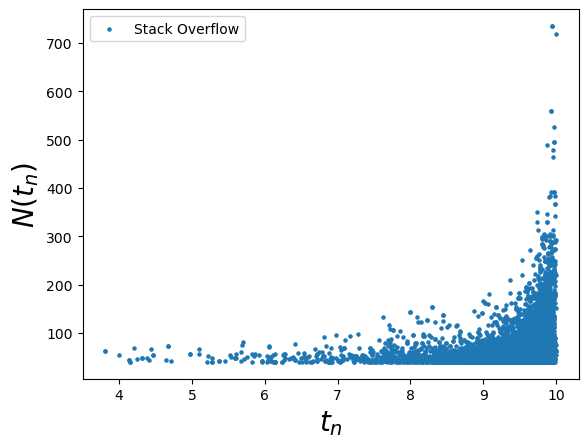}
    \end{subfigure}

    \caption{Scatterplots of time to last event ($t_n$) against number of events ($N(t_n)$).}
    \label{fig:scatterplots}
\end{figure}

Retirer grid et couleur rouge. 

\clearpage
\thispagestyle{empty}
\newgeometry{top=0.5cm,bottom=0.5cm}

\textbf{LastFM}

\begin{figure}[ht!]
        \centering
    \begin{subfigure}[b]{0.4\textwidth}
        \includegraphics[width=\textwidth]{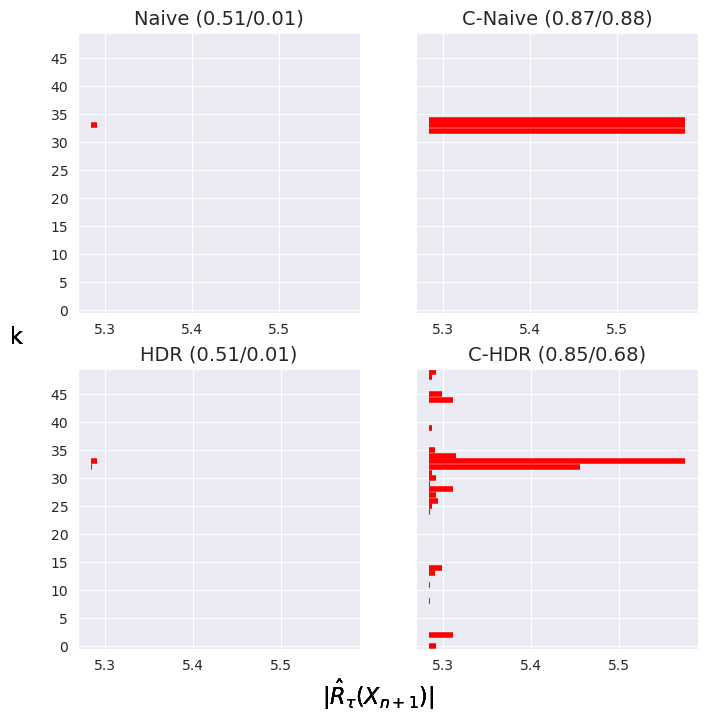}
    \end{subfigure}
    \begin{subfigure}[b]{0.4\textwidth}
        \includegraphics[width=\textwidth]{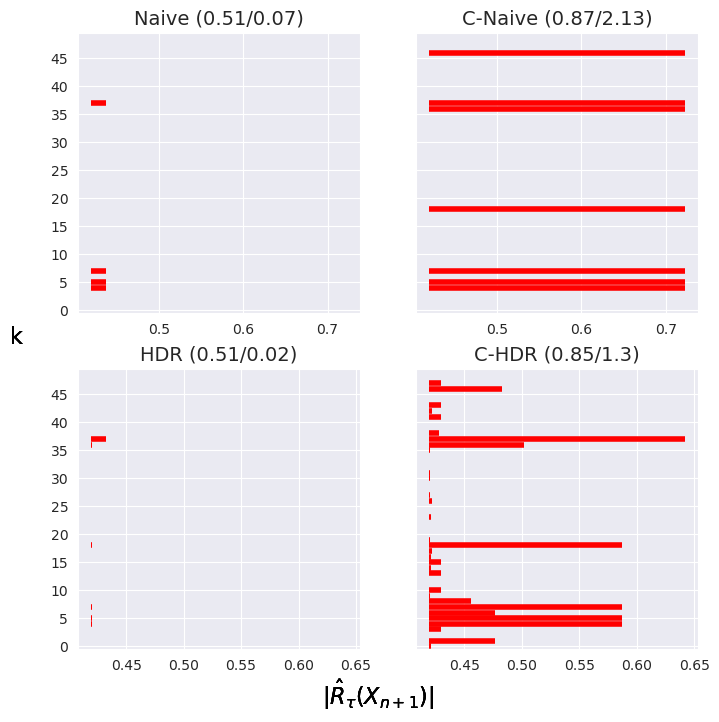}
    \end{subfigure}

    \begin{subfigure}[b]{0.4\textwidth}
        \includegraphics[width=\textwidth]{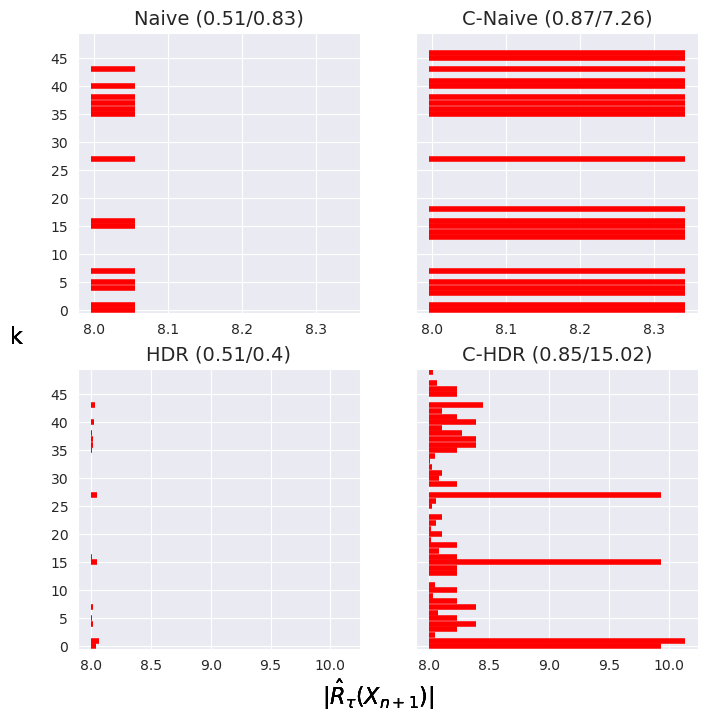}
    \end{subfigure}
    \begin{subfigure}[b]{0.4\textwidth}
        \includegraphics[width=\textwidth]{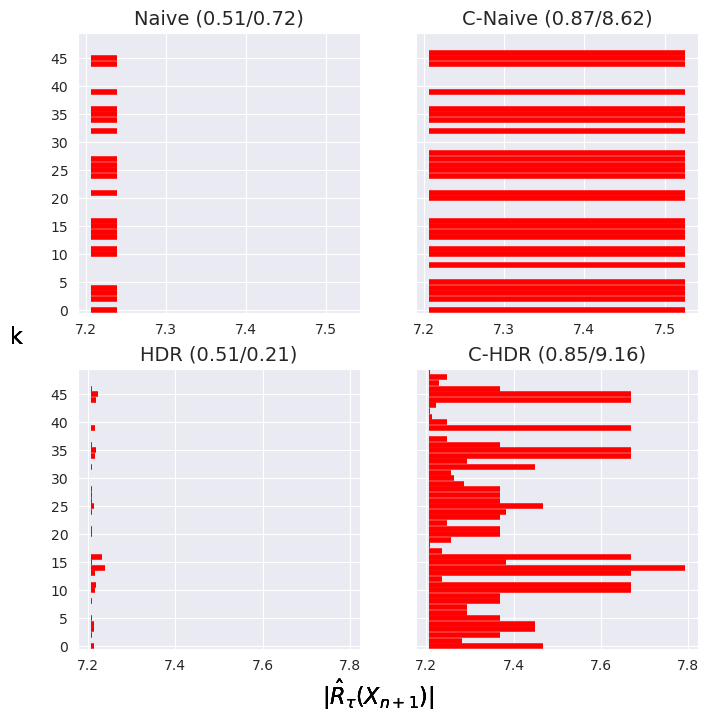}
    \end{subfigure}

    \begin{subfigure}[b]{0.4\textwidth}
        \includegraphics[width=\textwidth]{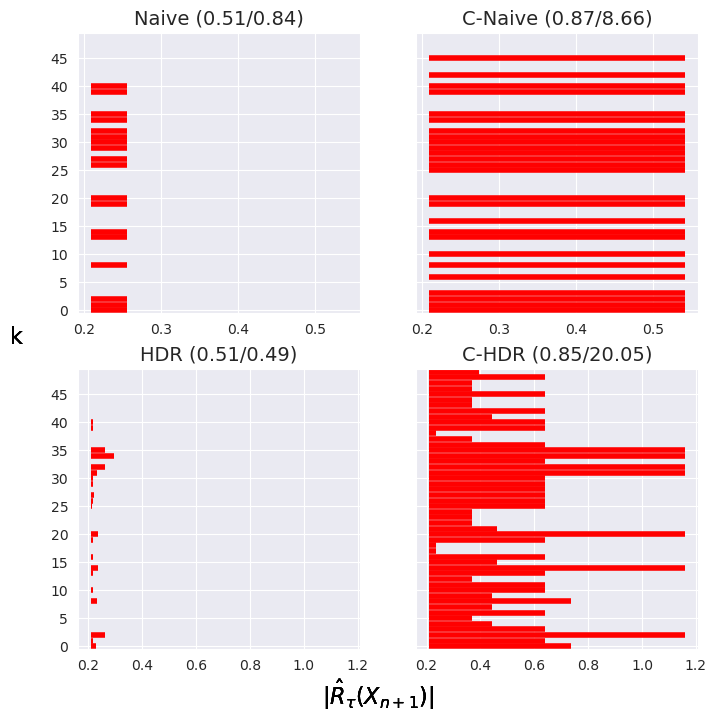}
    \end{subfigure}
    \begin{subfigure}[b]{0.4\textwidth}
        \includegraphics[width=\textwidth]{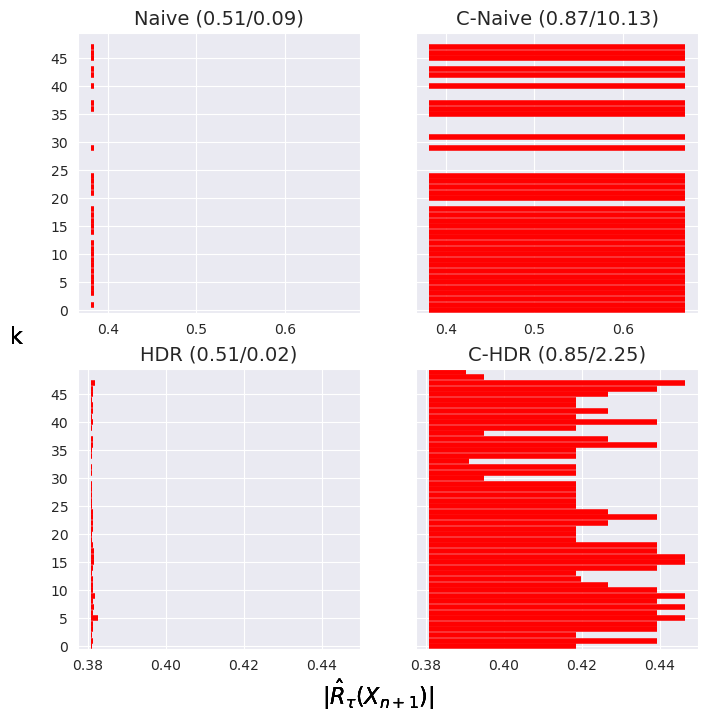}
    \end{subfigure}

    \begin{subfigure}[b]{0.4\textwidth}
        \includegraphics[width=\textwidth]{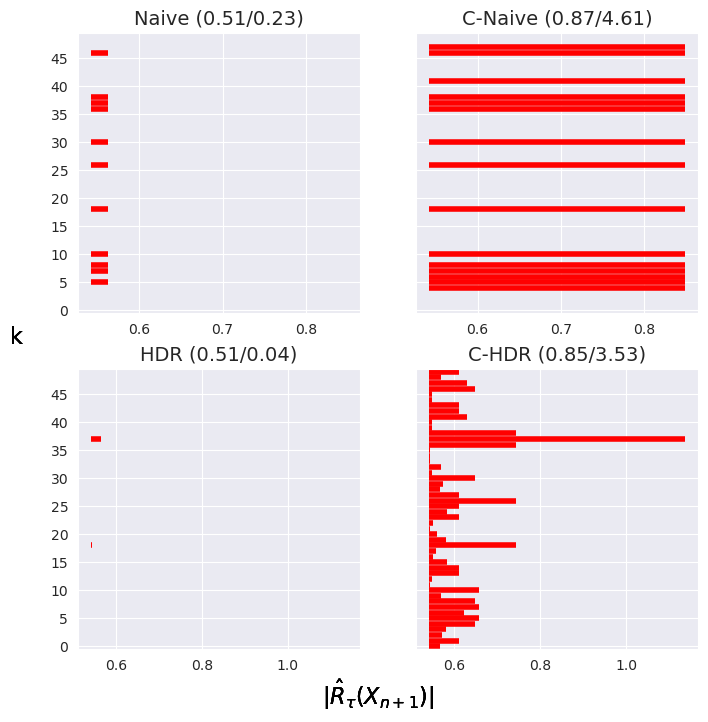}
    \end{subfigure}
    \begin{subfigure}[b]{0.4\textwidth}
        \includegraphics[width=\textwidth]{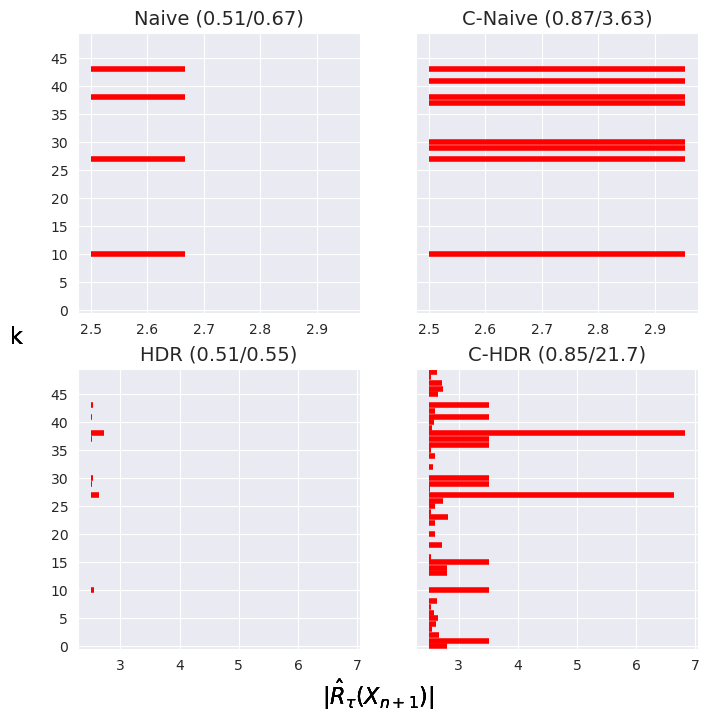}
    \end{subfigure}
    
\end{figure}

%%%%%%%%%%%%%%%%%%%%%%%%%%%%%%%%%%%%%%%%%%%%%%%%%%

\clearpage
\textbf{MOOC}

\begin{figure}[ht!]
        \centering
    \begin{subfigure}[b]{0.4\textwidth}
        \includegraphics[width=\textwidth]{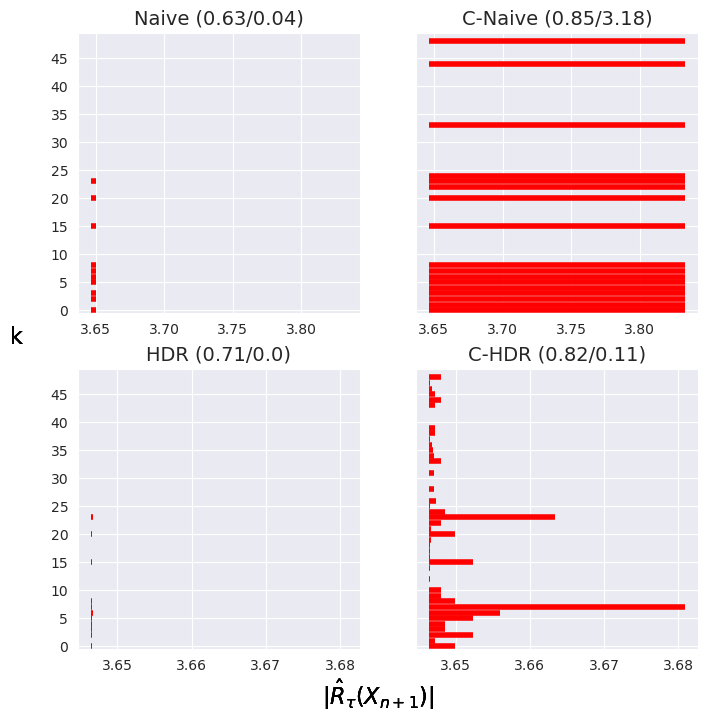}
    \end{subfigure}
    \begin{subfigure}[b]{0.4\textwidth}
        \includegraphics[width=\textwidth]{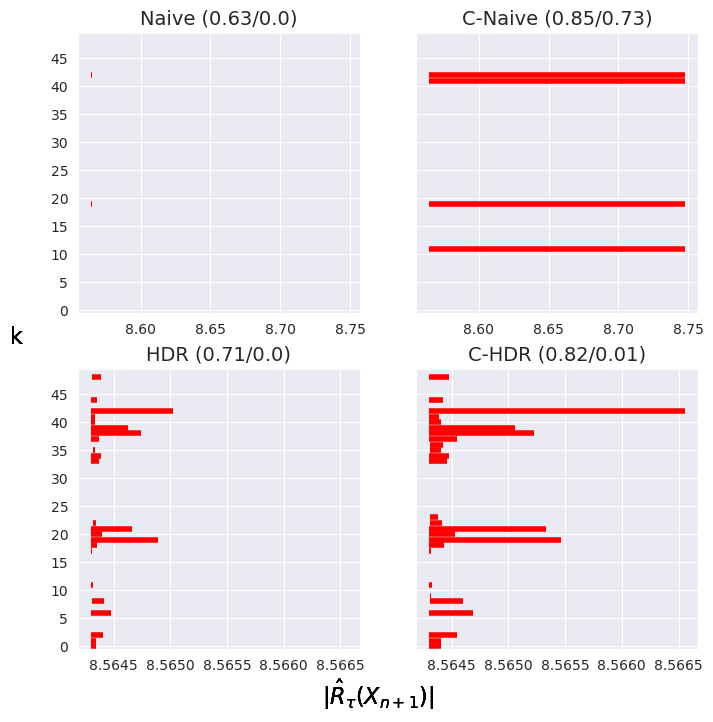}
    \end{subfigure}

    \begin{subfigure}[b]{0.4\textwidth}
        \includegraphics[width=\textwidth]{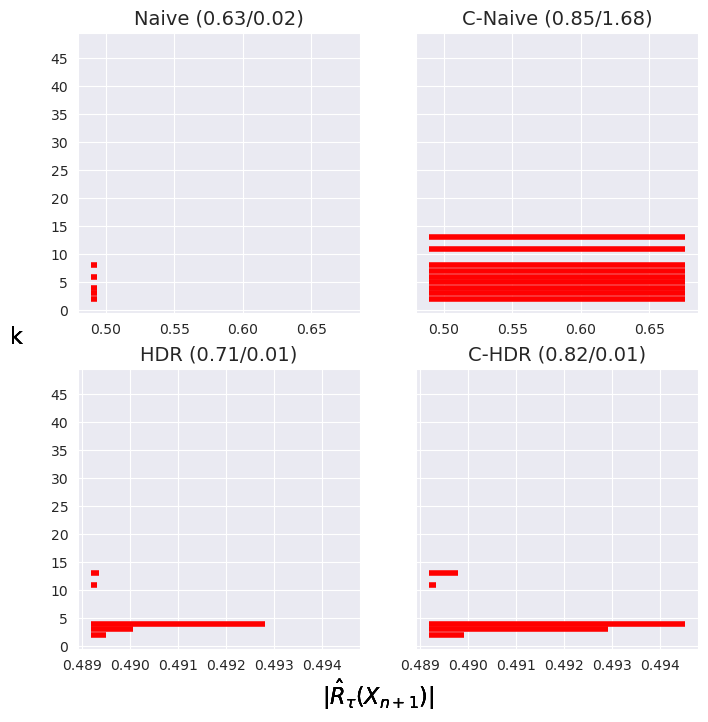}
    \end{subfigure}
    \begin{subfigure}[b]{0.4\textwidth}
        \includegraphics[width=\textwidth]{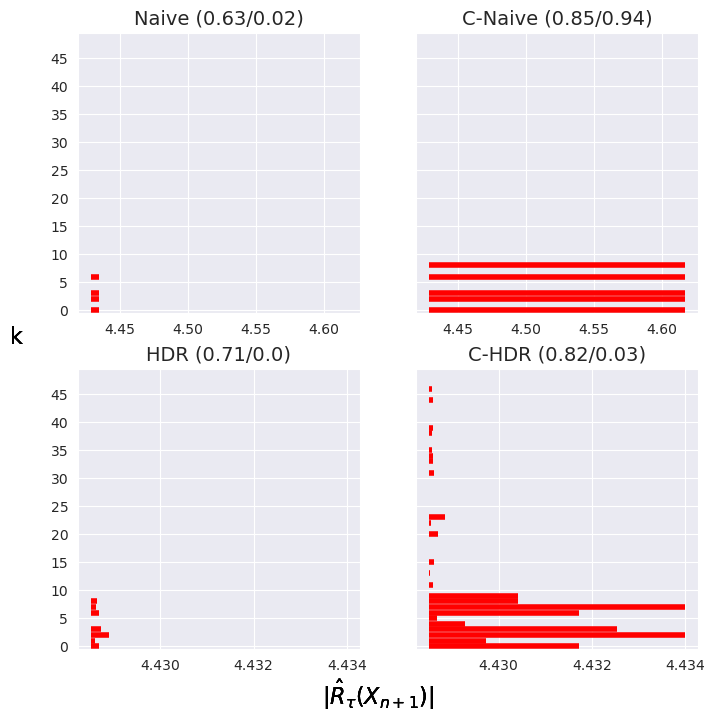}
    \end{subfigure}

    \begin{subfigure}[b]{0.4\textwidth}
        \includegraphics[width=\textwidth]{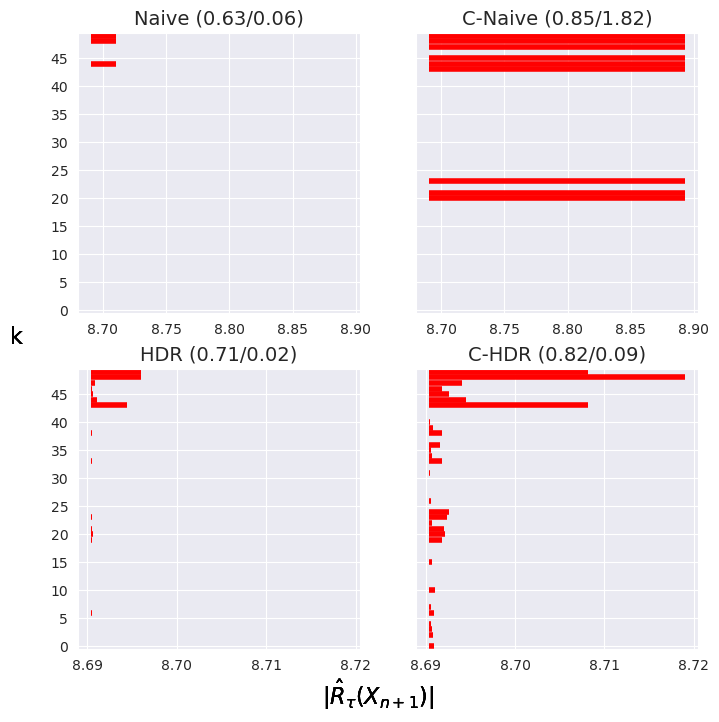}
    \end{subfigure}
    \begin{subfigure}[b]{0.4\textwidth}
        \includegraphics[width=\textwidth]{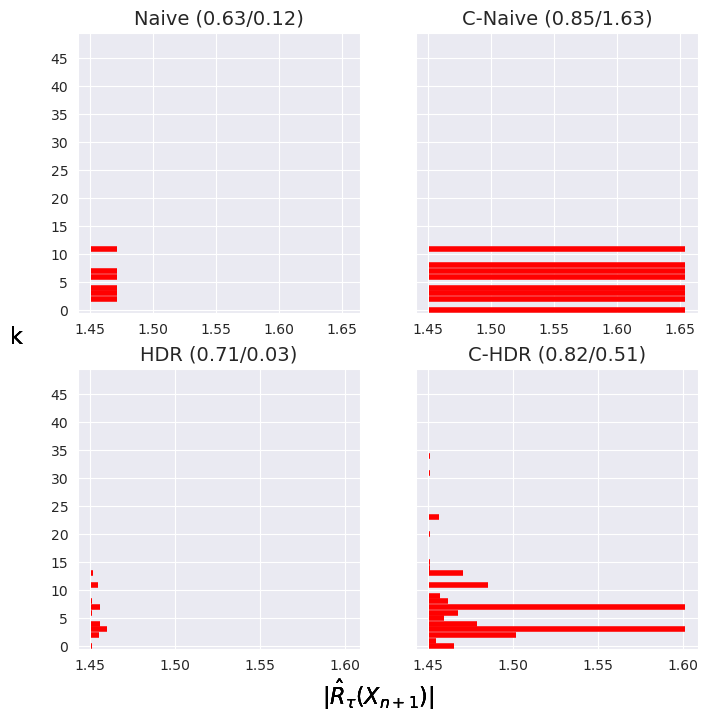}
    \end{subfigure}

    \begin{subfigure}[b]{0.4\textwidth}
        \includegraphics[width=\textwidth]{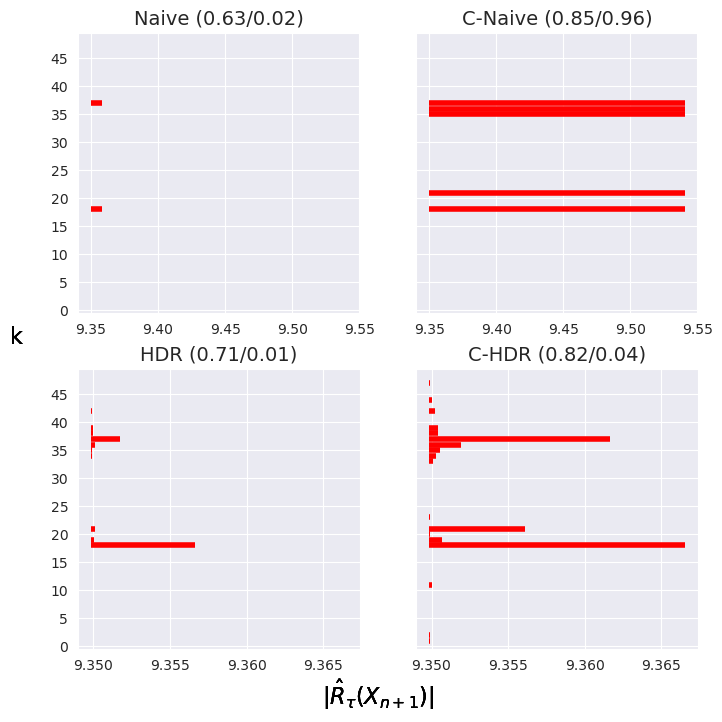}
    \end{subfigure}
    \begin{subfigure}[b]{0.4\textwidth}
        \includegraphics[width=\textwidth]{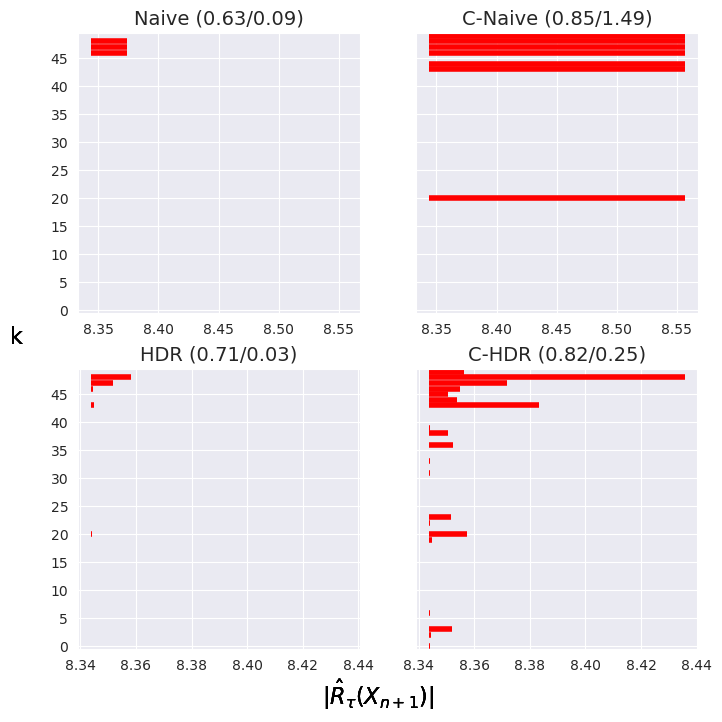}
    \end{subfigure}
    
\end{figure}

%%%%%%%%%%%%%%%%%%%%%%%%%%%%%%%%%%%%%%%%%%%%%%%%%%%%

\clearpage
\textbf{Github}

\begin{figure}[ht!]
        \centering
    \begin{subfigure}[b]{0.4\textwidth}
        \includegraphics[width=\textwidth]{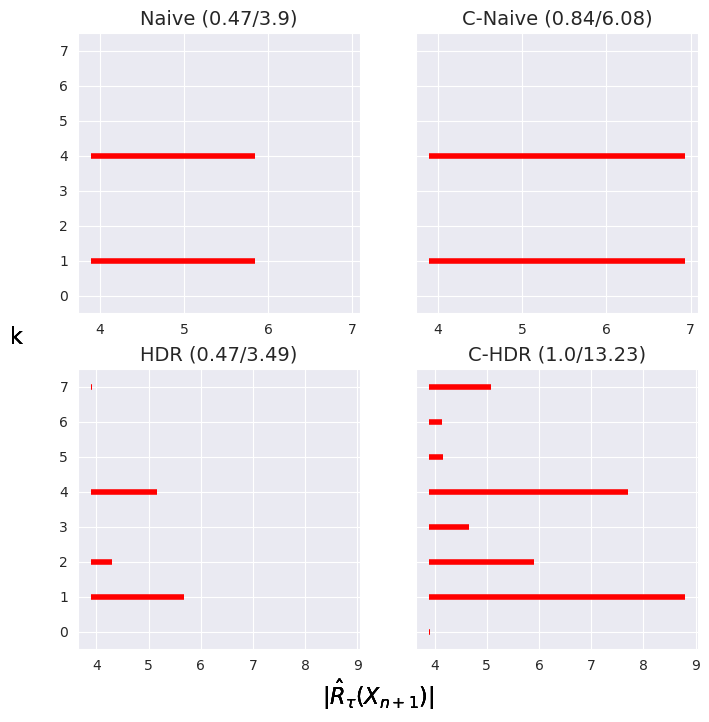}
    \end{subfigure}
    \begin{subfigure}[b]{0.4\textwidth}
        \includegraphics[width=\textwidth]{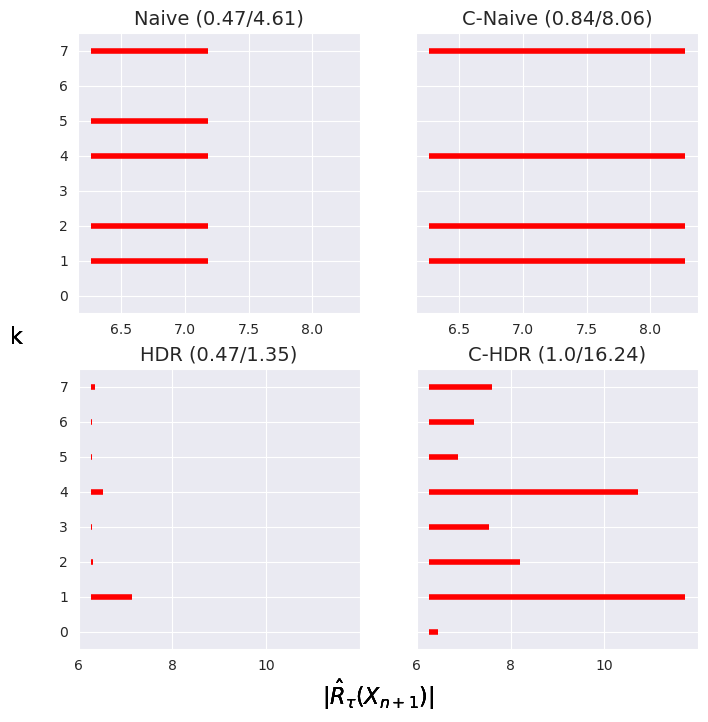}
    \end{subfigure}

    \begin{subfigure}[b]{0.4\textwidth}
        \includegraphics[width=\textwidth]{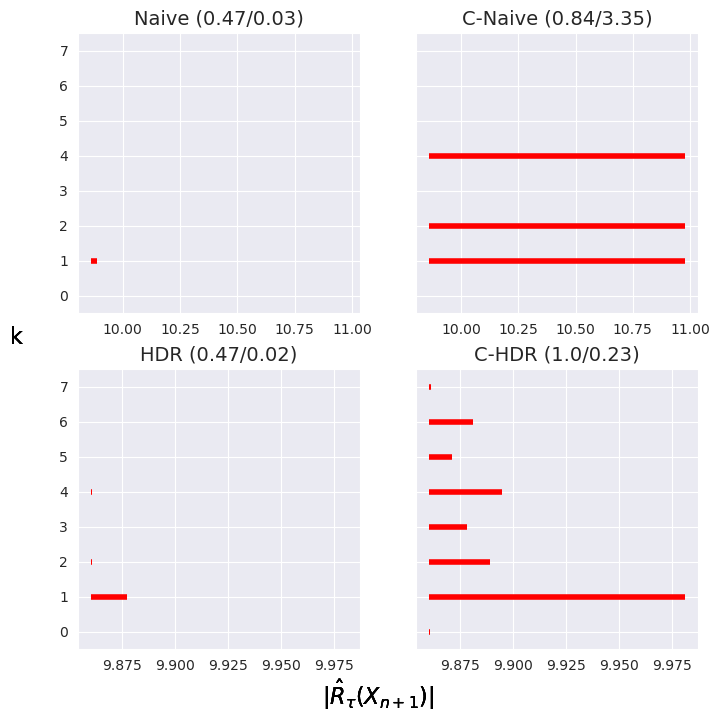}
    \end{subfigure}
    \begin{subfigure}[b]{0.4\textwidth}
        \includegraphics[width=\textwidth]{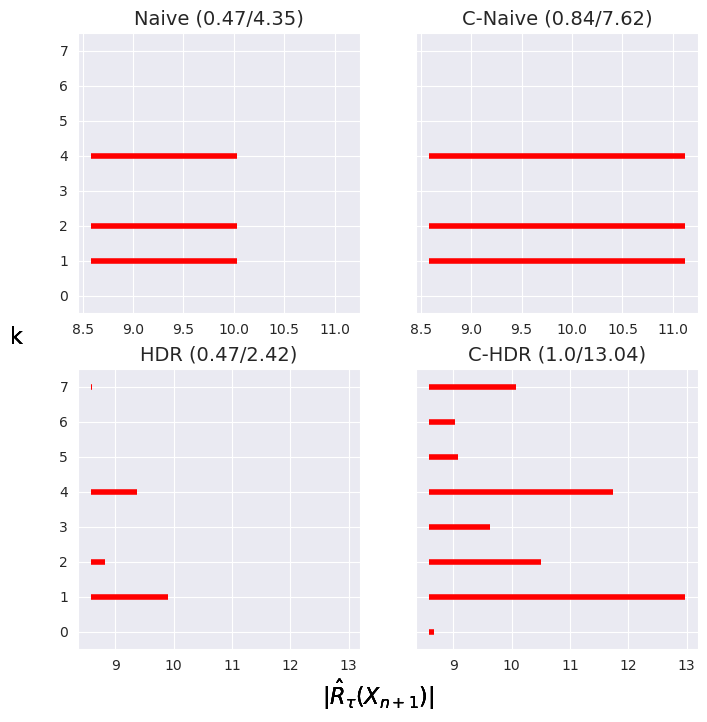}
    \end{subfigure}

    \begin{subfigure}[b]{0.4\textwidth}
        \includegraphics[width=\textwidth]{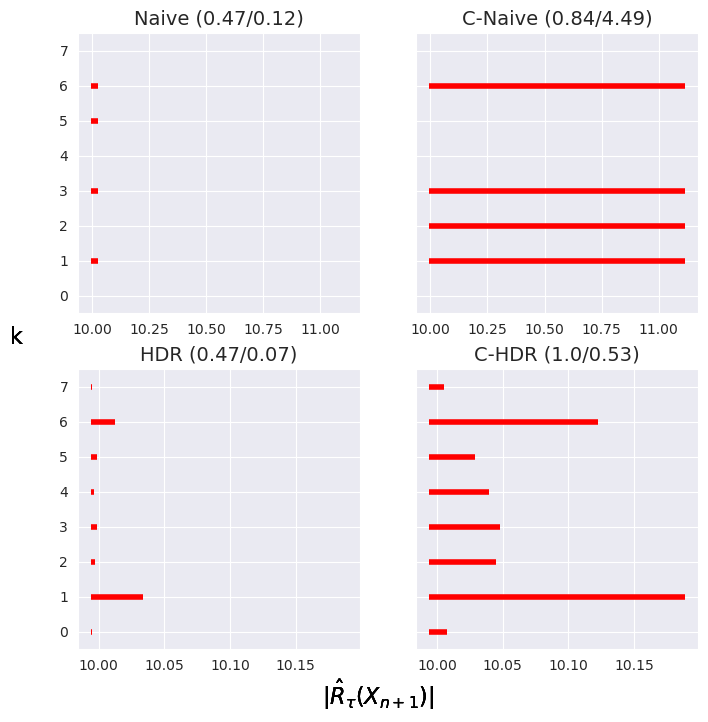}
    \end{subfigure}
    \begin{subfigure}[b]{0.4\textwidth}
        \includegraphics[width=\textwidth]{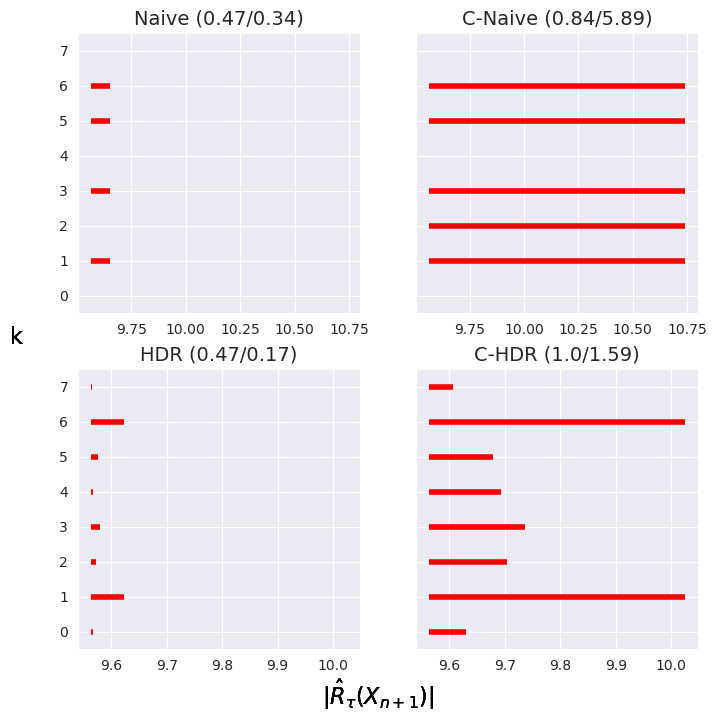}
    \end{subfigure}

    \begin{subfigure}[b]{0.4\textwidth}
        \includegraphics[width=\textwidth]{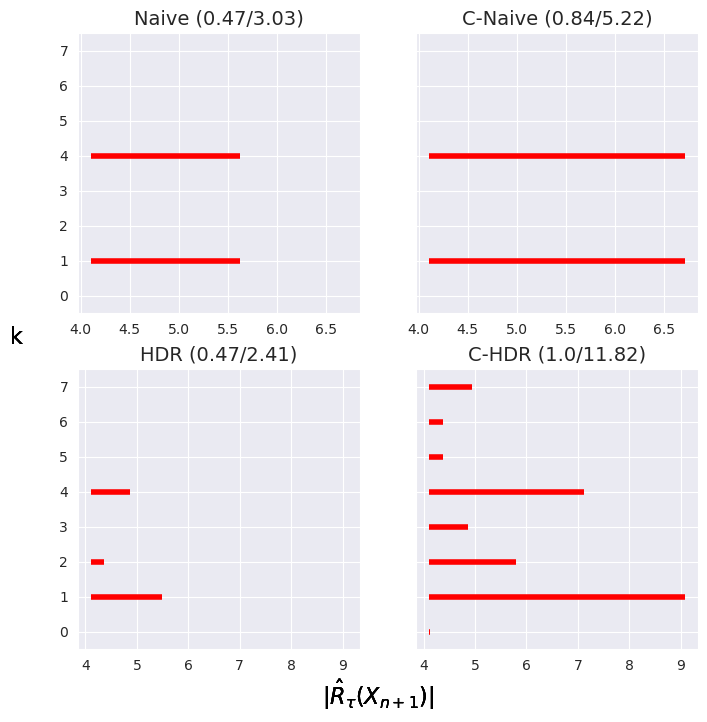}
    \end{subfigure}
    \begin{subfigure}[b]{0.4\textwidth}
        \includegraphics[width=\textwidth]{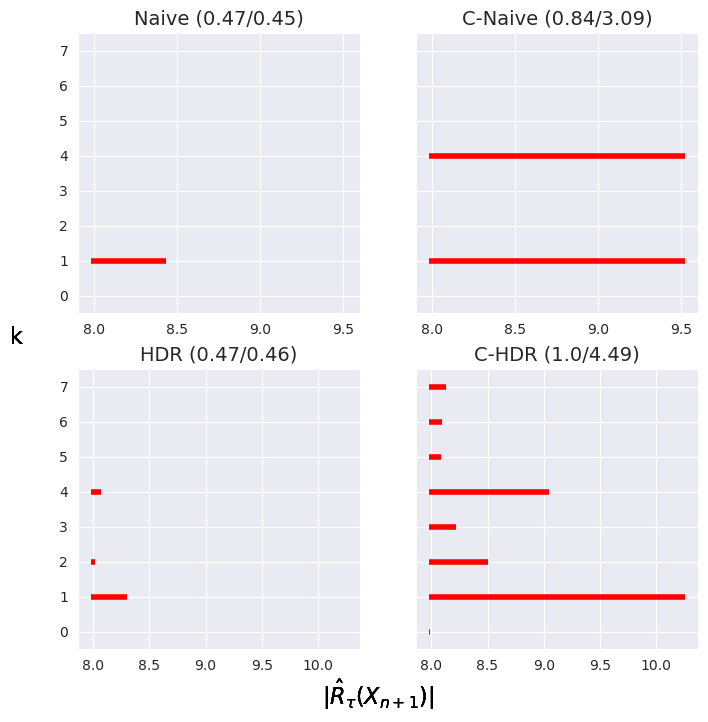}
    \end{subfigure}
    
\end{figure}

%%%%%%%%%%%%%%%%%%%%%%%%%%%%%%%%%%%%%%%%%%

\clearpage
\textbf{Reddit}

\begin{figure}[ht!]
        \centering
    \begin{subfigure}[b]{0.4\textwidth}
        \includegraphics[width=\textwidth]{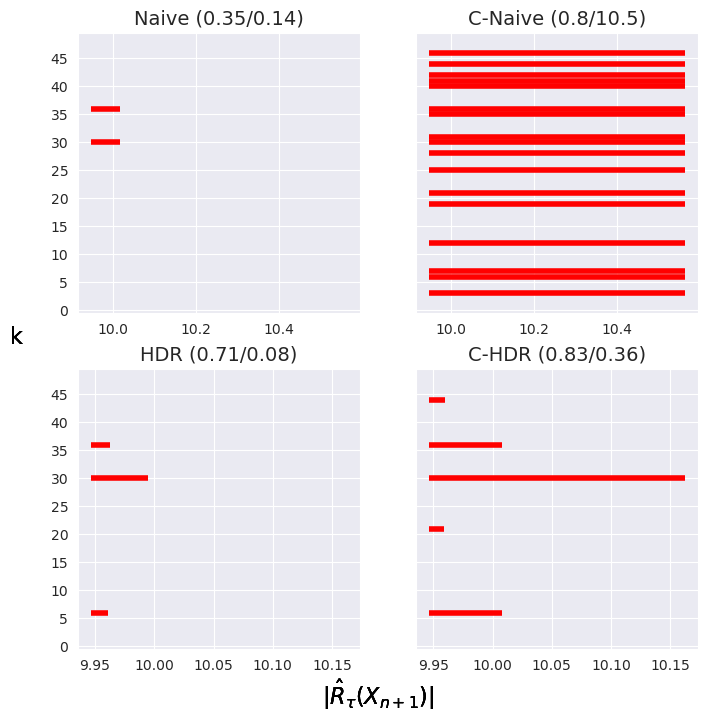}
    \end{subfigure}
    \begin{subfigure}[b]{0.4\textwidth}
        \includegraphics[width=\textwidth]{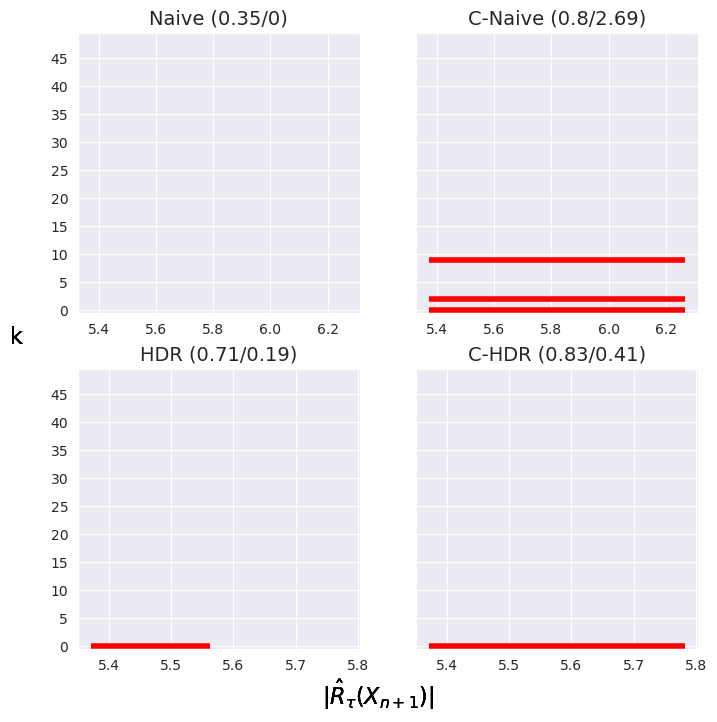}
    \end{subfigure}

    \begin{subfigure}[b]{0.4\textwidth}
        \includegraphics[width=\textwidth]{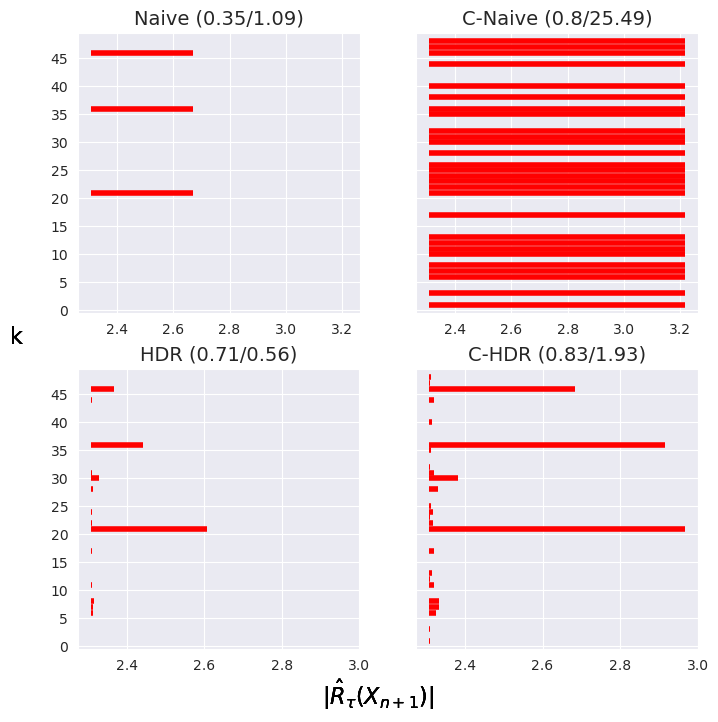}
    \end{subfigure}
    \begin{subfigure}[b]{0.4\textwidth}
        \includegraphics[width=\textwidth]{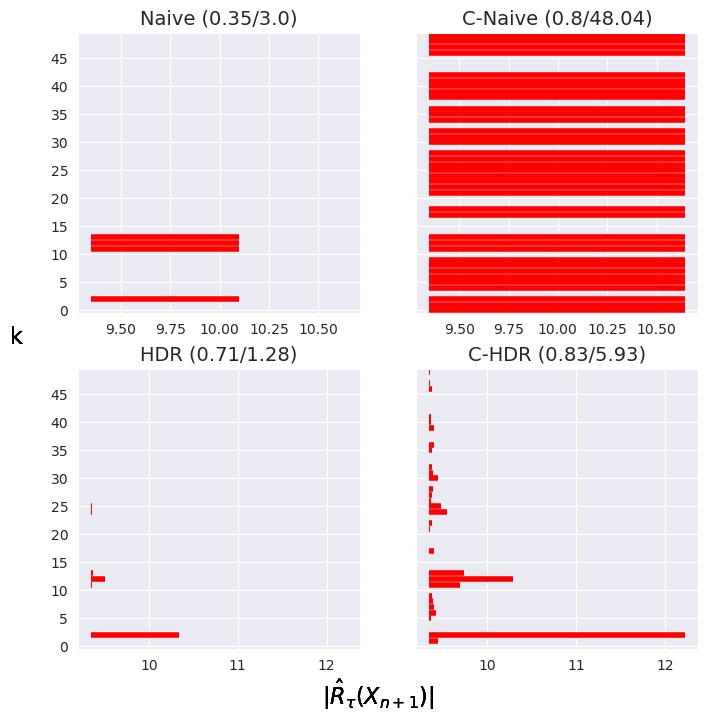}
    \end{subfigure}

    \begin{subfigure}[b]{0.4\textwidth}
        \includegraphics[width=\textwidth]{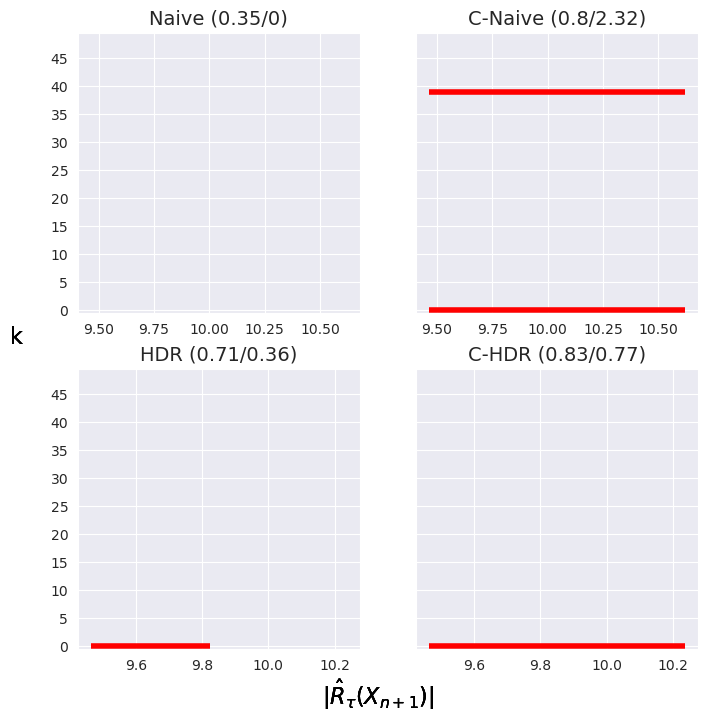}
    \end{subfigure}
    \begin{subfigure}[b]{0.4\textwidth}
        \includegraphics[width=\textwidth]{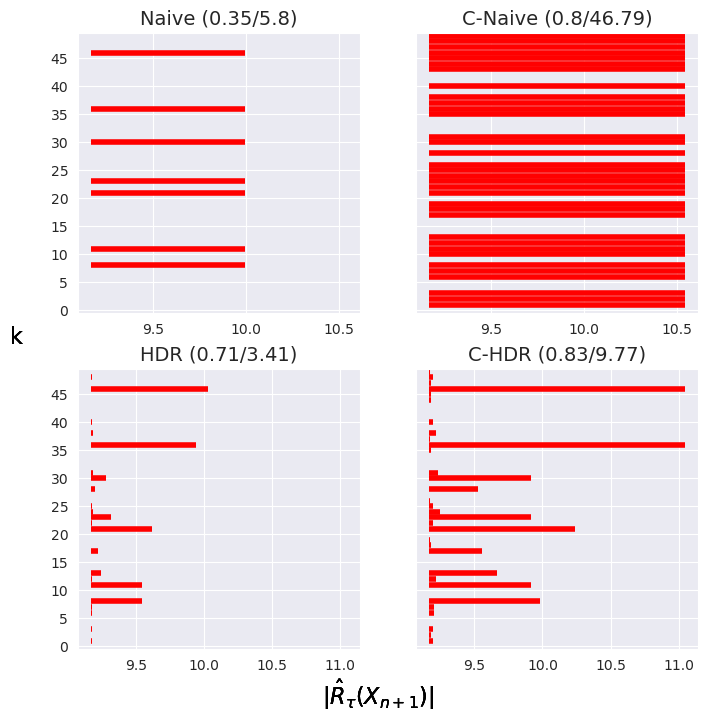}
    \end{subfigure}

    \begin{subfigure}[b]{0.4\textwidth}
        \includegraphics[width=\textwidth]{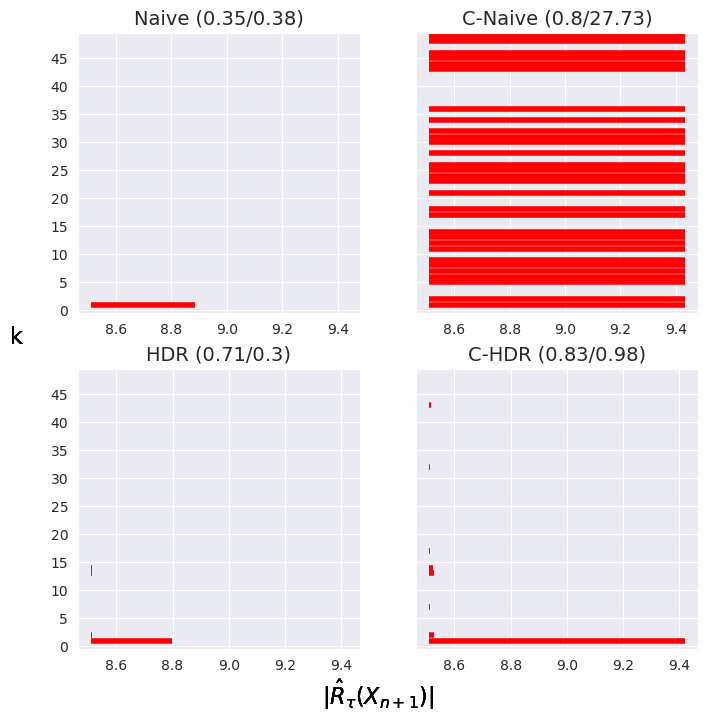}
    \end{subfigure}
    \begin{subfigure}[b]{0.4\textwidth}
        \includegraphics[width=\textwidth]{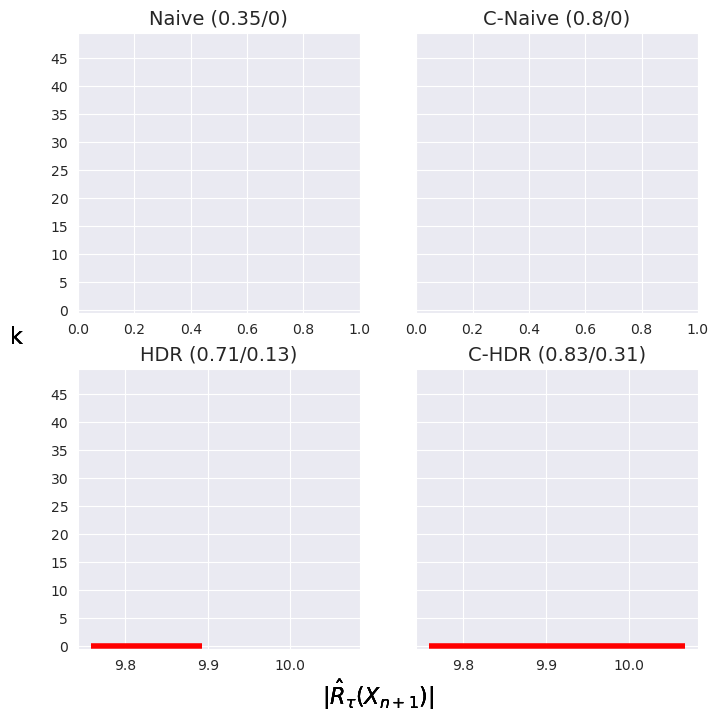}
    \end{subfigure}
    
\end{figure}

%%%%%%%%%%%%%%%%%%%%%%%%%%%%%%%%%%%%%%%%%%%%%%%%%%%

\clearpage
\textbf{Retweets}

\begin{figure}[ht!]
        \centering
    \begin{subfigure}[b]{0.4\textwidth}
        \includegraphics[width=\textwidth]{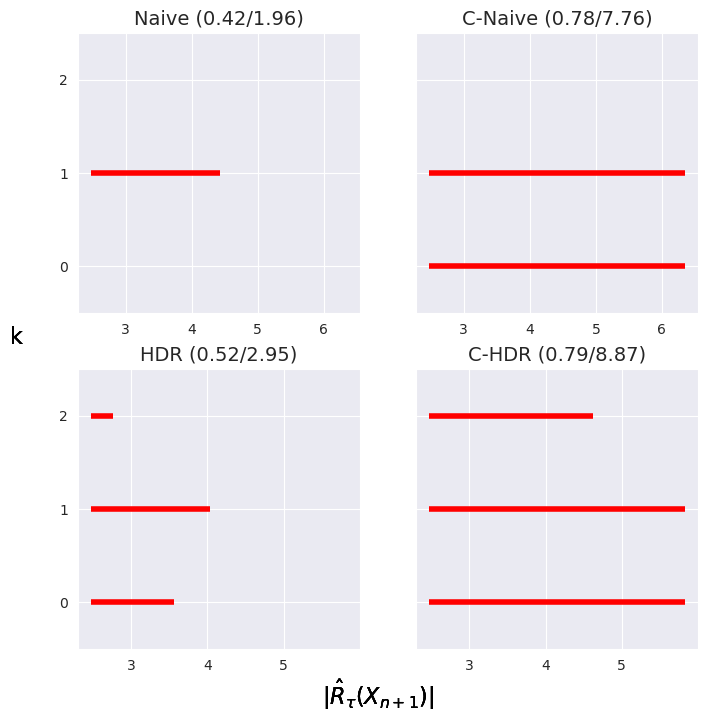}
    \end{subfigure}
    \begin{subfigure}[b]{0.4\textwidth}
        \includegraphics[width=\textwidth]{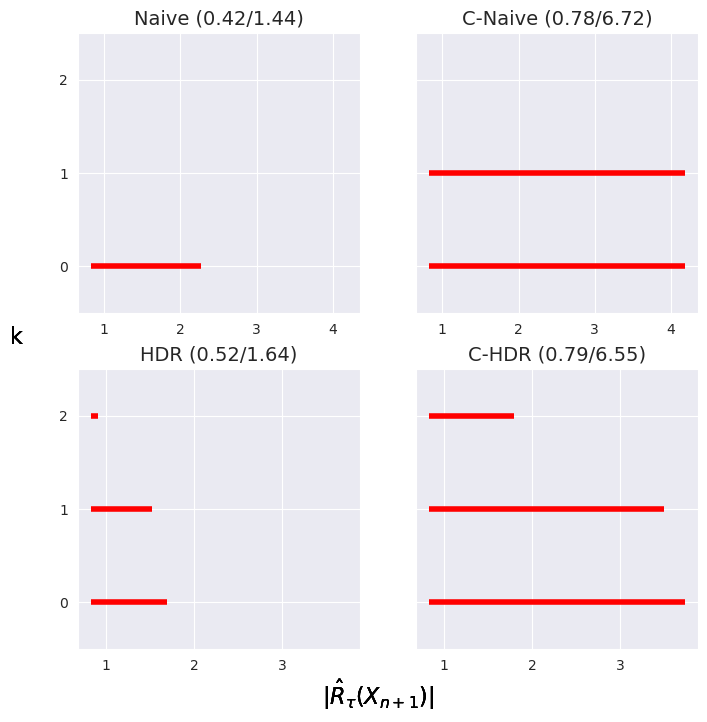}
    \end{subfigure}

    \begin{subfigure}[b]{0.4\textwidth}
        \includegraphics[width=\textwidth]{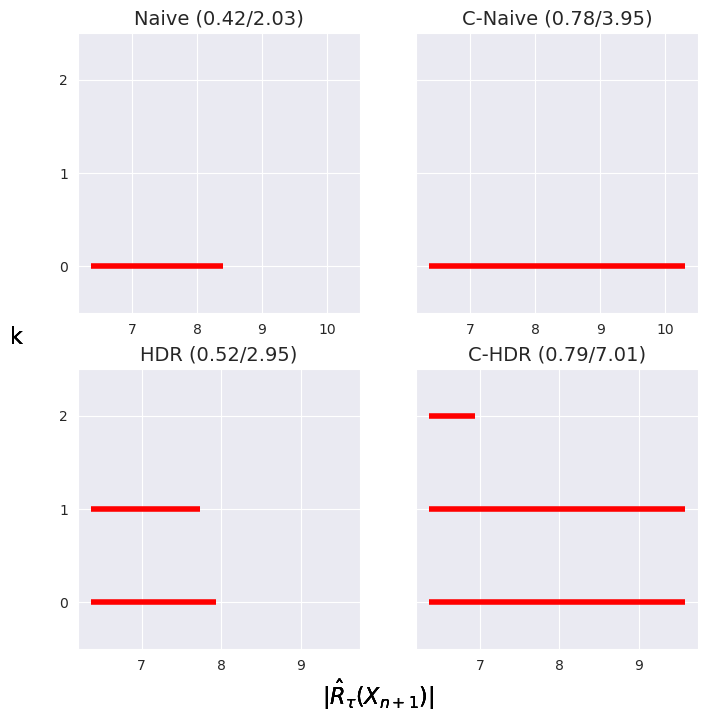}
    \end{subfigure}
    \begin{subfigure}[b]{0.4\textwidth}
        \includegraphics[width=\textwidth]{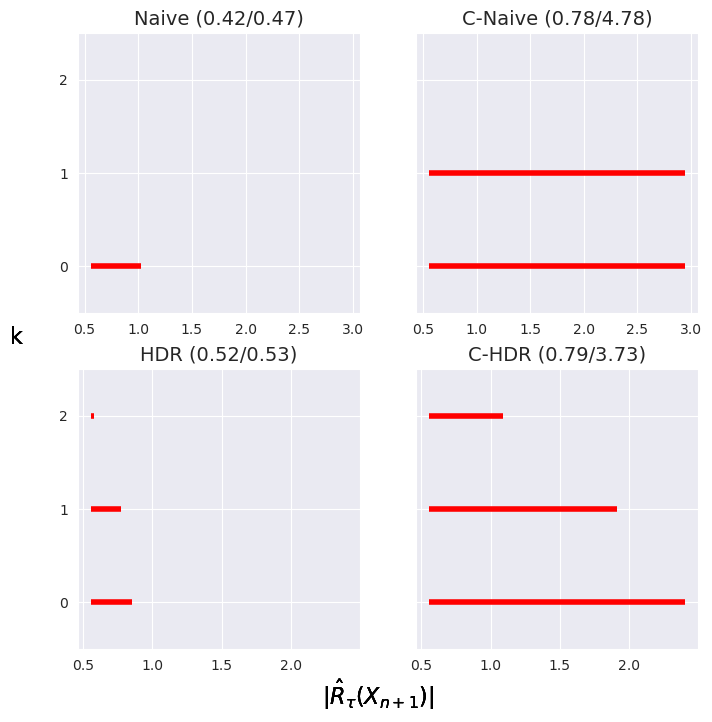}
    \end{subfigure}

    \begin{subfigure}[b]{0.4\textwidth}
        \includegraphics[width=\textwidth]{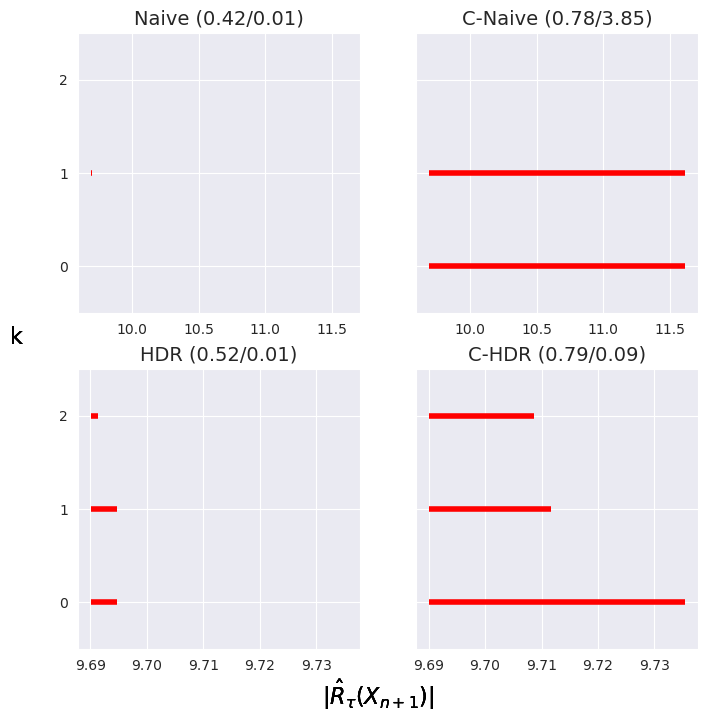}
    \end{subfigure}
    \begin{subfigure}[b]{0.4\textwidth}
        \includegraphics[width=\textwidth]{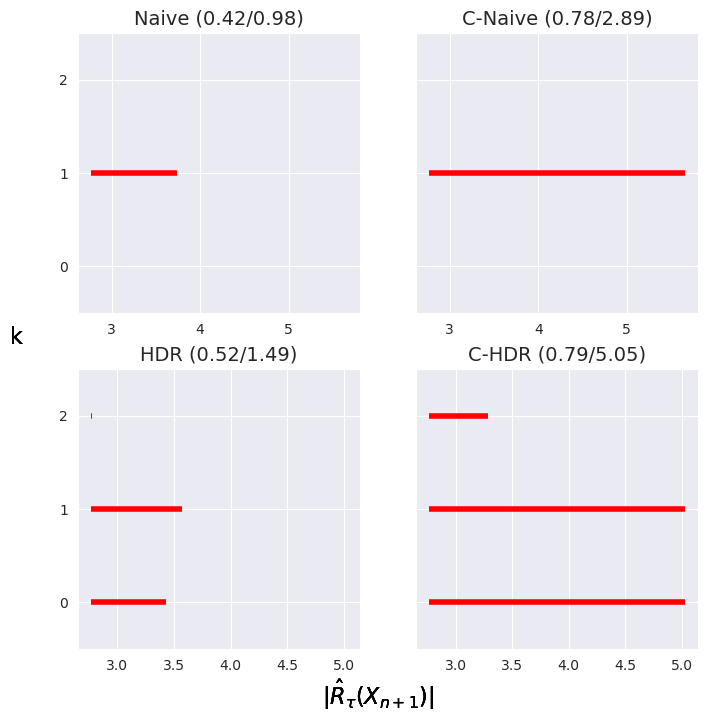}
    \end{subfigure}

    \begin{subfigure}[b]{0.4\textwidth}
        \includegraphics[width=\textwidth]{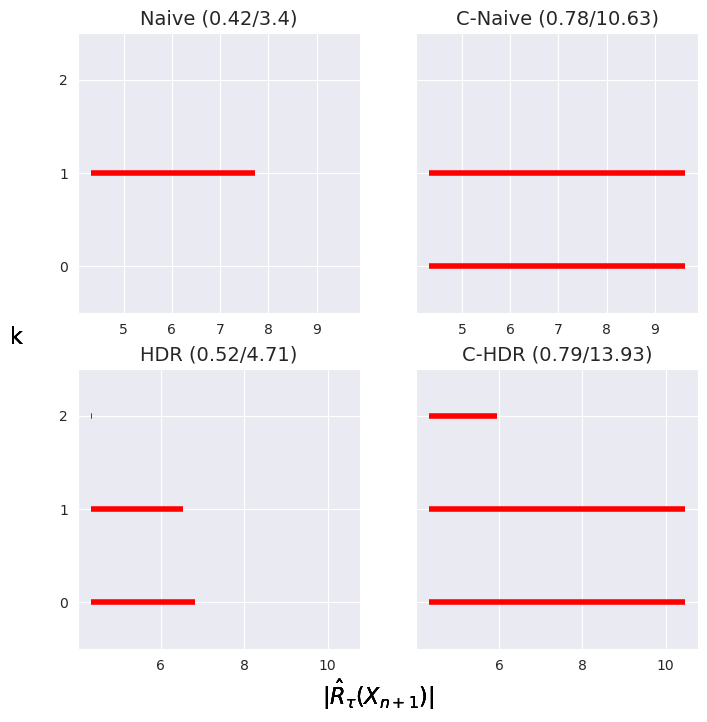}
    \end{subfigure}
    \begin{subfigure}[b]{0.4\textwidth}
        \includegraphics[width=\textwidth]{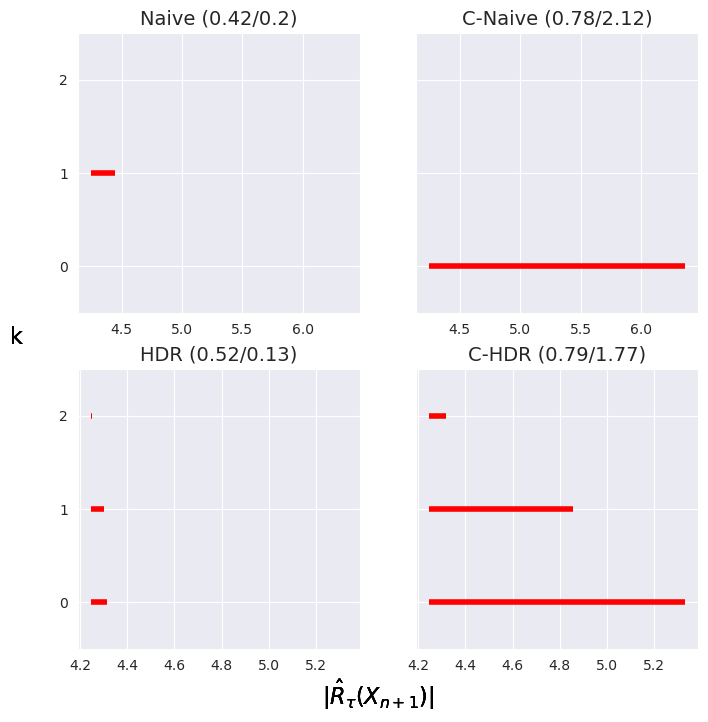}
    \end{subfigure}
    
\end{figure}

%%%%%%%%%%%%%%%%%%%%%%%%%%%%%%%%%%%%%%%%%%%%%%

\clearpage
\textbf{Stack Overflow}

\begin{figure}[ht!]
        \centering
    \begin{subfigure}[b]{0.4\textwidth}
        \includegraphics[width=\textwidth]{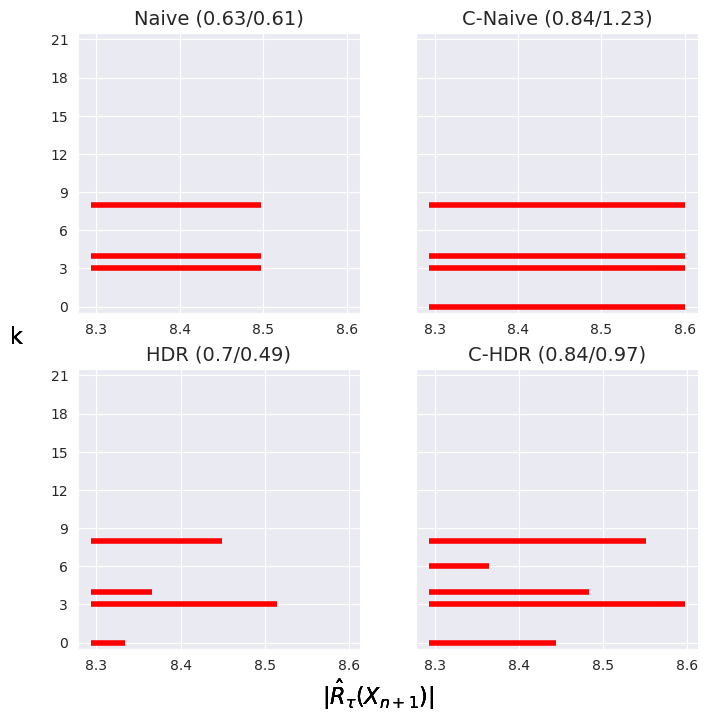}
    \end{subfigure}
    \begin{subfigure}[b]{0.4\textwidth}
        \includegraphics[width=\textwidth]{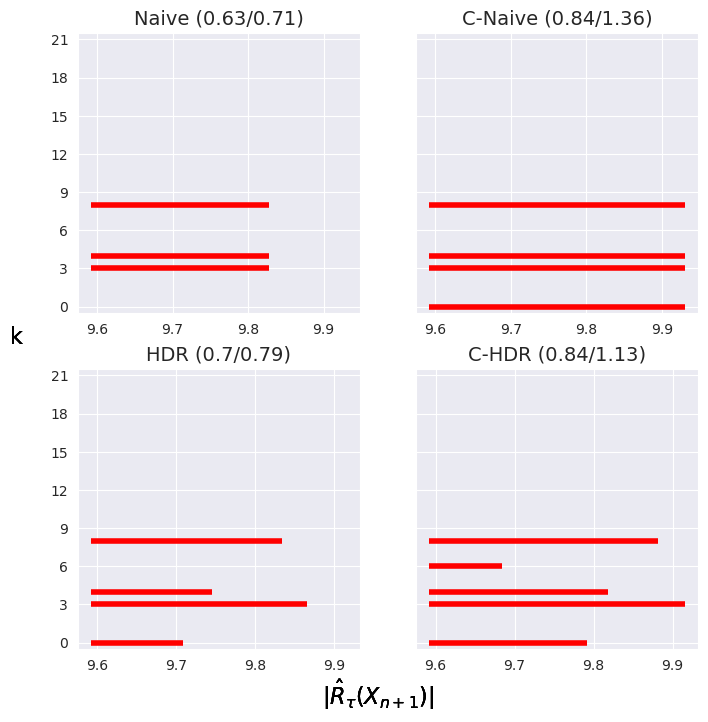}
    \end{subfigure}

    \begin{subfigure}[b]{0.4\textwidth}
        \includegraphics[width=\textwidth]{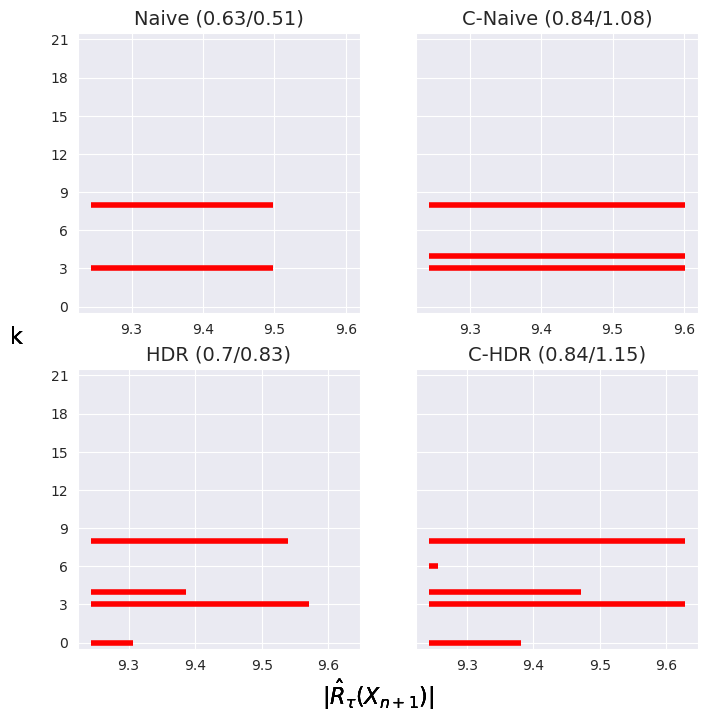}
    \end{subfigure}
    \begin{subfigure}[b]{0.4\textwidth}
        \includegraphics[width=\textwidth]{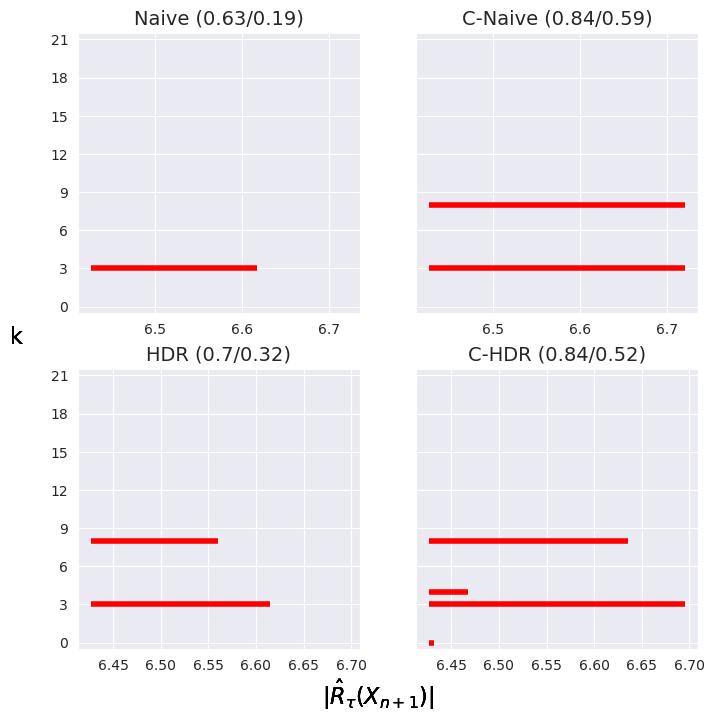}
    \end{subfigure}

    \begin{subfigure}[b]{0.4\textwidth}
        \includegraphics[width=\textwidth]{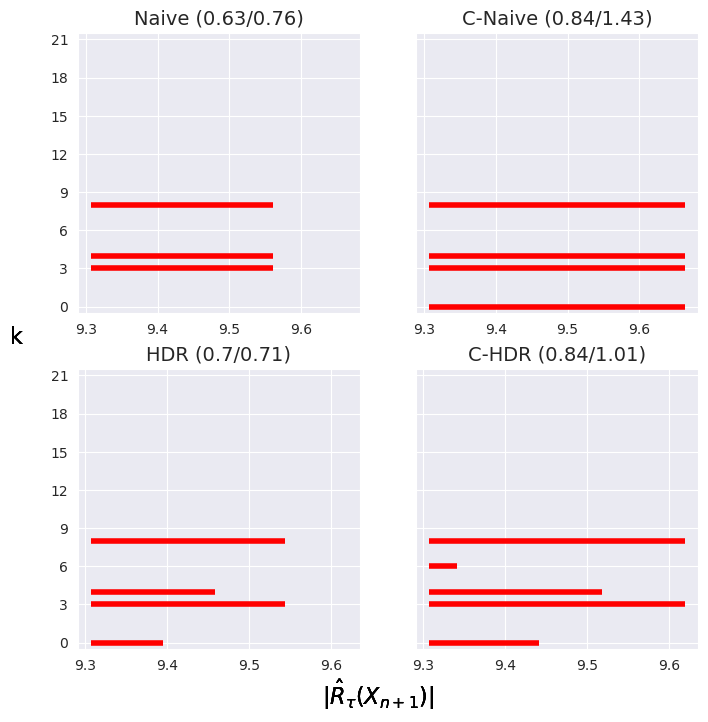}
    \end{subfigure}
    \begin{subfigure}[b]{0.4\textwidth}
        \includegraphics[width=\textwidth]{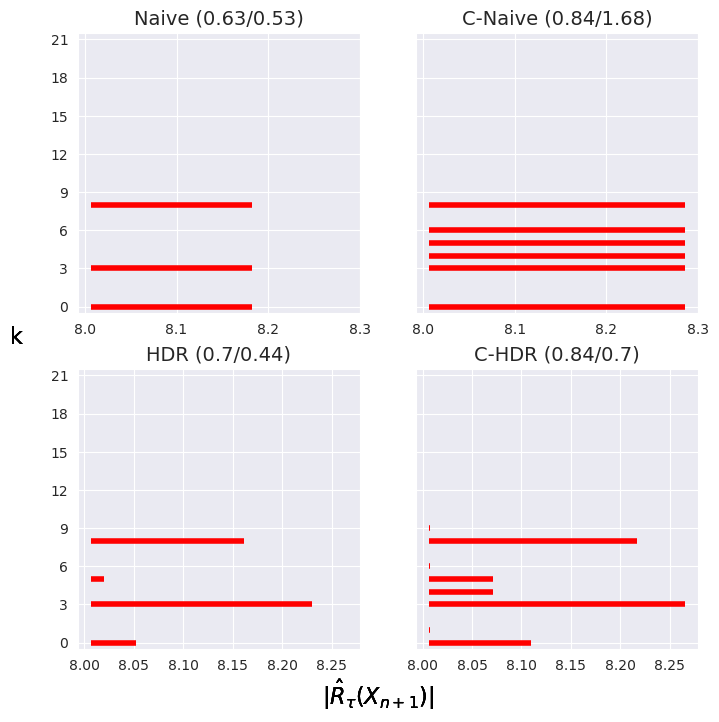}
    \end{subfigure}

    \begin{subfigure}[b]{0.4\textwidth}
        \includegraphics[width=\textwidth]{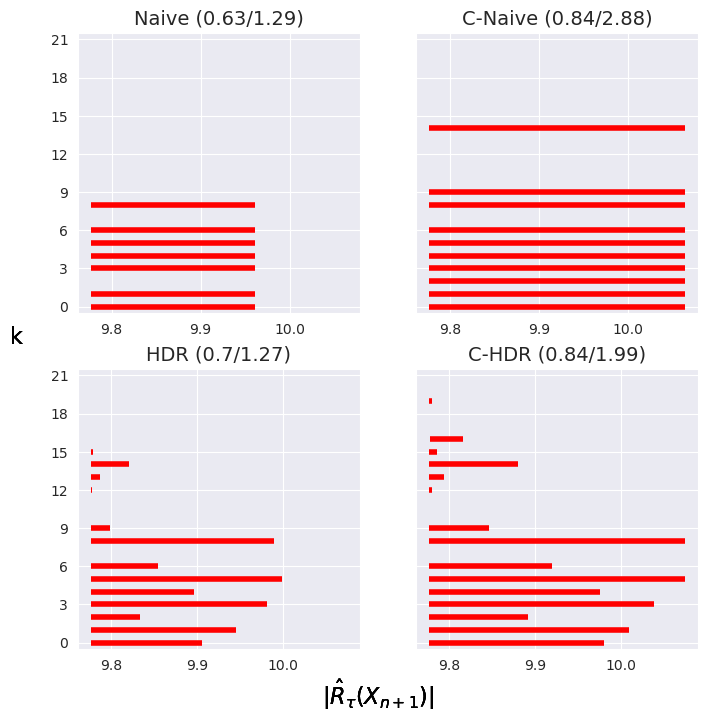}
    \end{subfigure}
    \begin{subfigure}[b]{0.4\textwidth}
        \includegraphics[width=\textwidth]{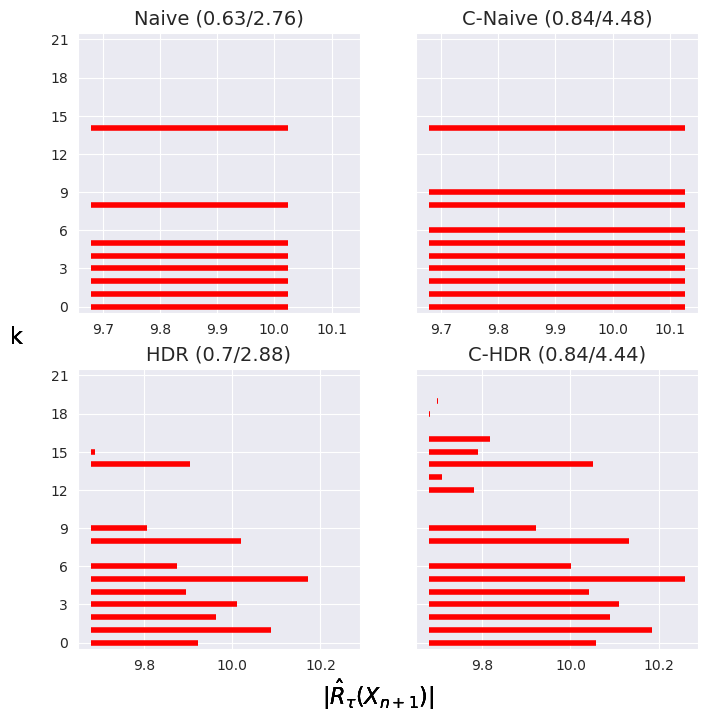}
    \end{subfigure}
    
\end{figure}

\restoregeometry

\clearpage
\thispagestyle{empty}
\newgeometry{top=0.5cm,bottom=0.5cm, left=0.5cm, right=0.5cm}

\begin{table}[h!]
\setlength\tabcolsep{1.5pt}
\small
\caption{Average coverage and length of the prediction regions generated by the Naive, Naive-C, HDR and C-HDR methods for various models and datasets.}
\begin{tabular}{cccccccc}
\toprule
                           & \multicolumn{7}{c}{Coverage} \\
                           & C-ConstAll & C-ConstAPS & C-CQRAll & Naive & C-Naive &   HDR & C-HDR \\
\midrule
        ('CLNM', 'LastFM') &      0.839 &      0.874 &    0.839 & 0.506 &   0.874 & 0.529 & 0.839 \\
          ('CLNM', 'MOOC') &       0.81 &       0.85 &    0.812 & 0.637 &   0.814 & 0.708 & 0.824 \\
        ('CLNM', 'Github') &      0.895 &      0.895 &    0.737 & 0.474 &   0.842 & 0.474 & 0.842 \\
        ('CLNM', 'Reddit') &      0.833 &      0.814 &     0.84 & 0.347 &   0.809 &  0.73 & 0.826 \\
      ('CLNM', 'Retweets') &      0.792 &      0.786 &    0.779 &  0.43 &   0.788 & 0.525 & 0.793 \\
('CLNM', 'Stack Overflow') &      0.801 &      0.828 &    0.803 & 0.619 &   0.847 & 0.693 &  0.82 \\
         ('THP', 'LastFM') &      0.839 &      0.862 &    0.839 & 0.494 &   0.862 & 0.494 & 0.793 \\
           ('THP', 'MOOC') &       0.81 &      0.847 &     0.81 & 0.809 &   0.848 & 0.697 & 0.666 \\
         ('THP', 'Github') &      0.895 &      0.947 &    0.895 & 0.368 &   0.947 & 0.368 & 0.579 \\
         ('THP', 'Reddit') &      0.833 &      0.823 &    0.833 & 0.133 &   0.823 & 0.314 & 0.498 \\
       ('THP', 'Retweets') &      0.792 &      0.792 &    0.792 & 0.356 &   0.793 &  0.48 & 0.746 \\
 ('THP', 'Stack Overflow') &      0.801 &      0.826 &    0.801 & 0.402 &   0.826 & 0.421 & 0.788 \\
\bottomrule
\toprule
                           & \multicolumn{7}{c}{Length} \\
                           & C-ConstAll & C-ConstAPS & C-CQRAll & Naive & C-Naive &   HDR &  C-HDR \\
\midrule
        ('CLNM', 'LastFM') &      8.054 &        6.7 &    8.083 & 0.734 &   \textbf{6.675} & 0.377 & 33.723 \\
          ('CLNM', 'MOOC') &      0.343 &      2.765 &    0.956 & 0.566 &   2.281 & 0.054 &  \textbf{0.255} \\
        ('CLNM', 'Github') &     16.299 &     10.622 &    8.046 & 1.608 &   5.968 & 1.197 &  \textbf{4.507} \\
        ('CLNM', 'Reddit') &     40.411 &     34.417 &   36.916 &   3.6 &  30.713 & 2.351 &  \textbf{6.025} \\
      ('CLNM', 'Retweets') &      6.793 &      6.712 &     \textbf{6.04} & 1.612 &   \textbf{6.042} & 1.932 &  6.465 \\
('CLNM', 'Stack Overflow') &      6.051 &       2.41 &    5.978 & 1.087 &   2.194 & 1.065 &  \textbf{1.653} \\
         ('THP', 'LastFM') &      8.054 &      9.805 &    8.054 & 1.093 &  10.068 & 0.961 &  \textbf{4.684} \\
           ('THP', 'MOOC') &      0.343 &      2.233 &    0.343 & 0.329 &   2.243 & 0.292 &  \textbf{0.255} \\
         ('THP', 'Github') &     16.299 &     14.468 &   16.299 & 0.788 &  14.468 & 0.761 &   3.85 \\
         ('THP', 'Reddit') &     40.411 &     28.739 &   40.411 & 0.182 &  28.735 & 0.165 &  1.647 \\
       ('THP', 'Retweets') &      6.793 &      6.724 &    6.799 & 0.888 &   6.729 & 1.328 &  5.761 \\
 ('THP', 'Stack Overflow') &      6.051 &      2.147 &    6.051 & 0.436 &   2.144 & 0.412 &  2.329 \\
\bottomrule
\toprule
                           & \multicolumn{7}{c}{WSC} \\
                           & C-ConstAll & C-ConstAPS & C-CQRAll & Naive & C-Naive &   HDR & C-HDR \\
\midrule
        ('CLNM', 'LastFM') &        0.6 &      0.857 &      0.9 & 0.333 &    0.75 &   0.4 & 0.818 \\
          ('CLNM', 'MOOC') &      0.776 &      0.826 &    0.843 & 0.667 &   0.836 & 0.623 & 0.803 \\
        ('CLNM', 'Github') &        1.0 &        1.0 &      1.0 &   0.4 &    0.75 & 0.667 &   1.0 \\
        ('CLNM', 'Reddit') &      0.652 &      0.595 &    0.679 &  0.06 &   0.568 &  0.75 & \textbf{0.868} \\
      ('CLNM', 'Retweets') &      0.685 &      0.766 &    0.795 & 0.403 &   0.795 & 0.482 & 0.748 \\
('CLNM', 'Stack Overflow') &      0.609 &      0.732 &    0.696 & 0.538 &   \textbf{0.807} & 0.716 & 0.758 \\
         ('THP', 'LastFM') &        1.0 &        1.0 &    0.875 &   0.4 &   0.857 & 0.417 & 0.786 \\
           ('THP', 'MOOC') &      0.874 &      0.778 &    0.885 & 0.795 &   0.861 & 0.754 & 0.636 \\
         ('THP', 'Github') &        nan &        1.0 &      1.0 &   0.6 &     1.0 &  0.75 & 0.667 \\
         ('THP', 'Reddit') &       0.86 &      0.562 &     0.61 & 0.161 &   0.577 & 0.337 & 0.515 \\
       ('THP', 'Retweets') &      0.688 &      0.776 &    0.648 & 0.224 &   0.777 & 0.289 & 0.673 \\
 ('THP', 'Stack Overflow') &      0.703 &      0.808 &     0.69 &  0.28 &   0.816 & 0.277 & 0.746 \\
\bottomrule
\end{tabular}

\end{table}

\restoregeometry
%%===========================================================================================%%
%% If you are submitting to one of the Nature Portfolio journals, using the eJP submission   %%
%% system, please include the references within the manuscript file itself. You may do this  %%
%% by copying the reference list from your .bbl file, paste it into the main manuscript .tex %%
%% file, and delete the associated \verb+\bibliography+ commands.                            %%
%%===================================================================================
\appendix

\section{Previous results}

\subsection{Time}

\begin{figure}[h!]
    \centering
    \includegraphics[width=\linewidth]{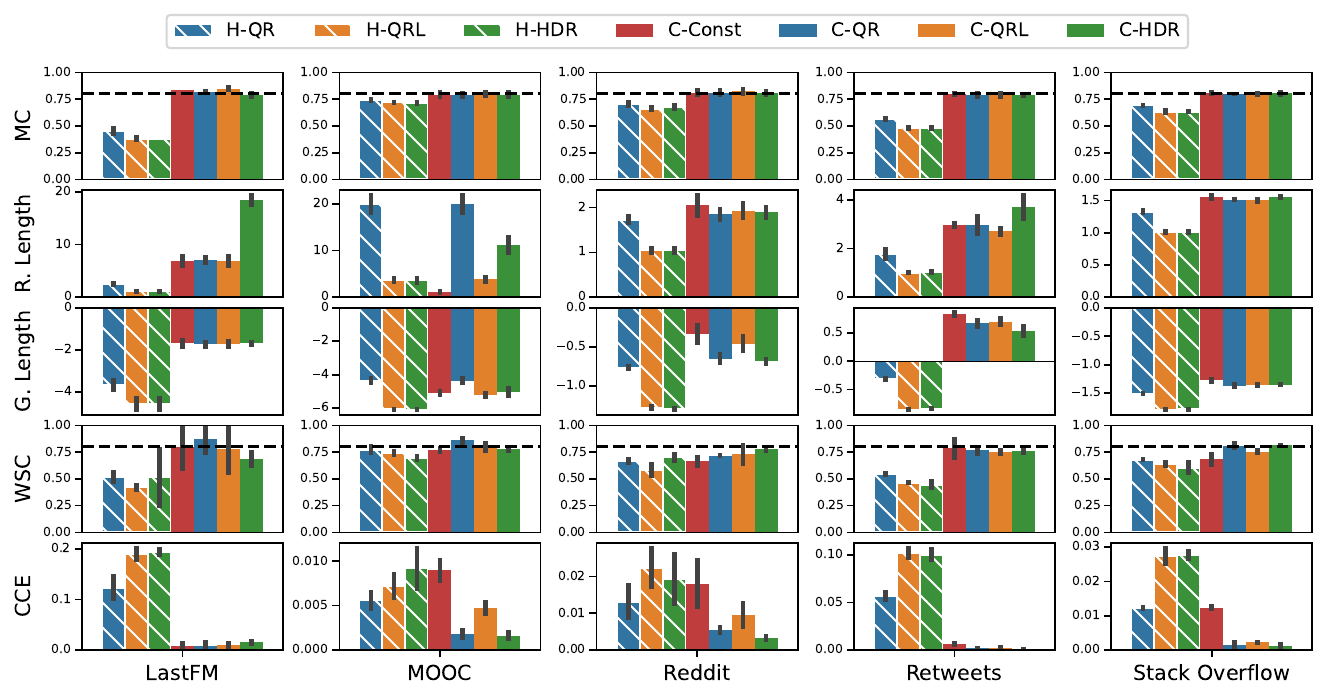}
    \caption{Performance of all methods on real world datasets using the CLNM model. Non-conformal methods are hatched. As expected, all conformal methods achieve marginal coverage. All conformal methods also achieve a relatively good conditional coverage. The size of the prediction region is indicated relative to the smallest run for each dataset and model. C-HDR achieves the smallest prediction region size except for LastFM and Retweets.}
\end{figure}

\begin{figure}[h!]
    \centering
    \includegraphics[width=\linewidth]{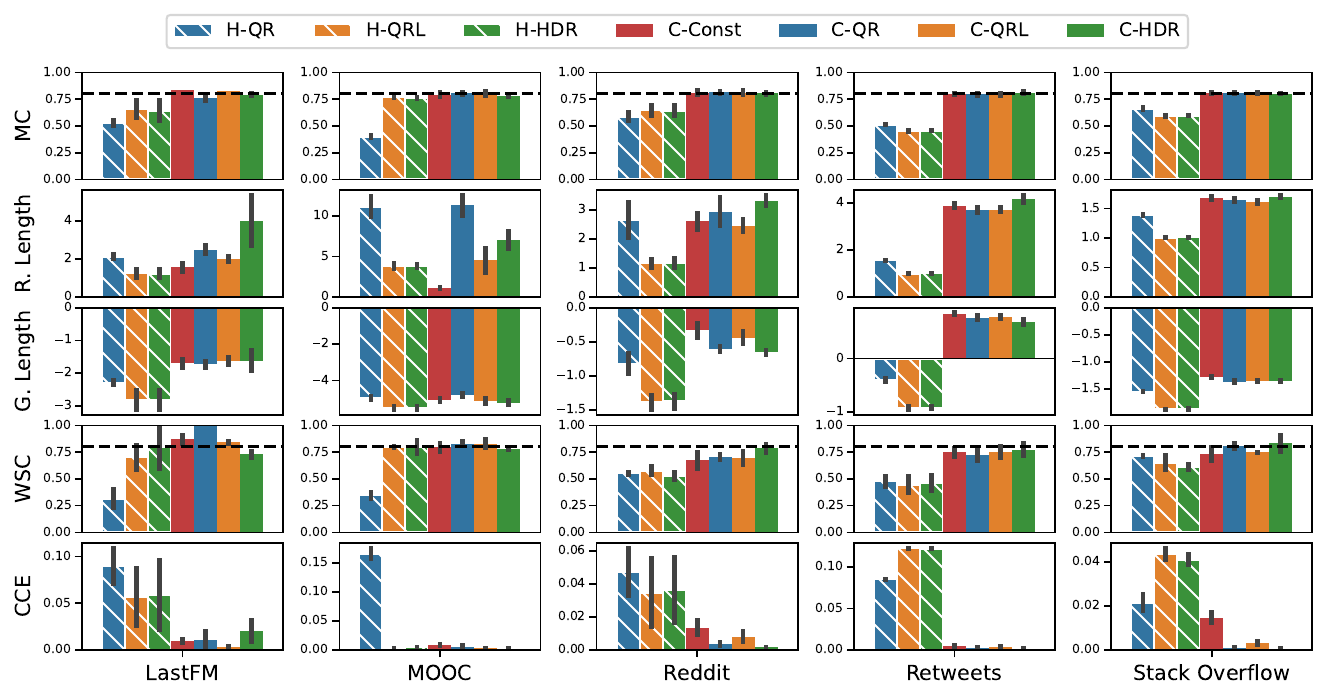}
    \caption{RMTPP}
\end{figure}

\begin{figure}[h!]
    \centering
    \includegraphics[width=\linewidth]{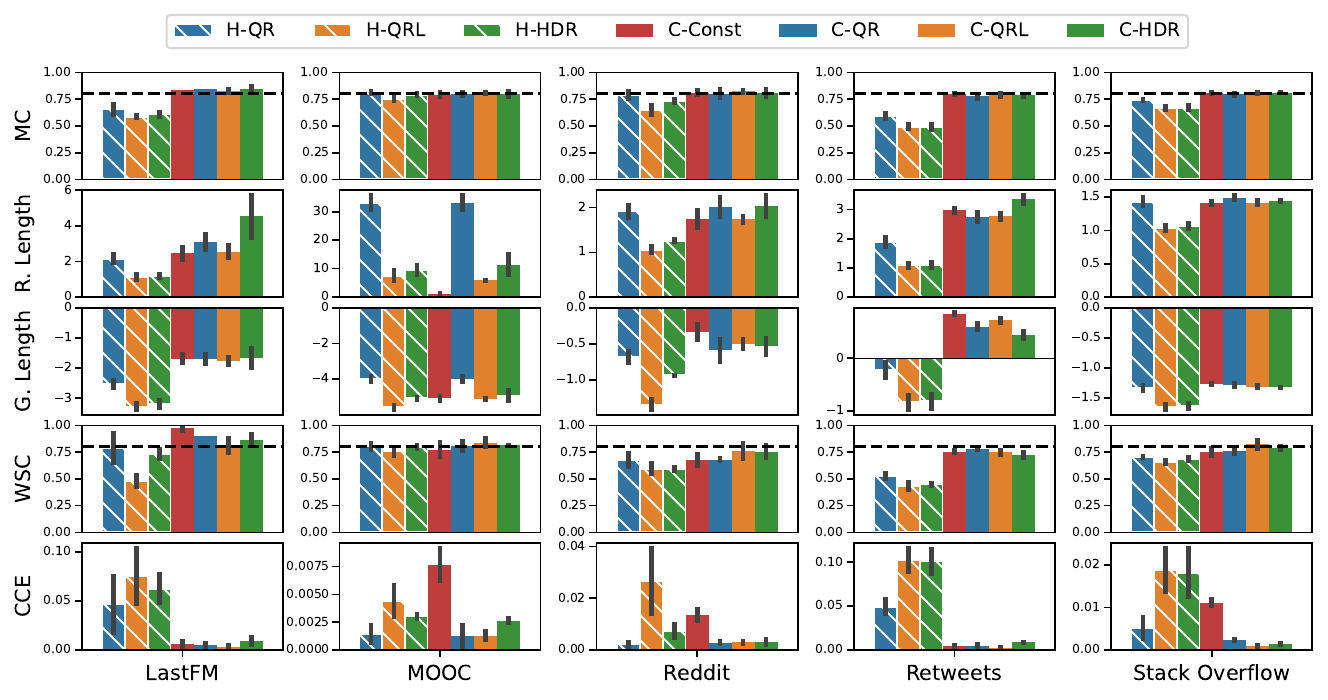}
    \caption{FNN}
\end{figure}

\begin{figure}[h!]
    \centering
    \includegraphics[width=\linewidth]{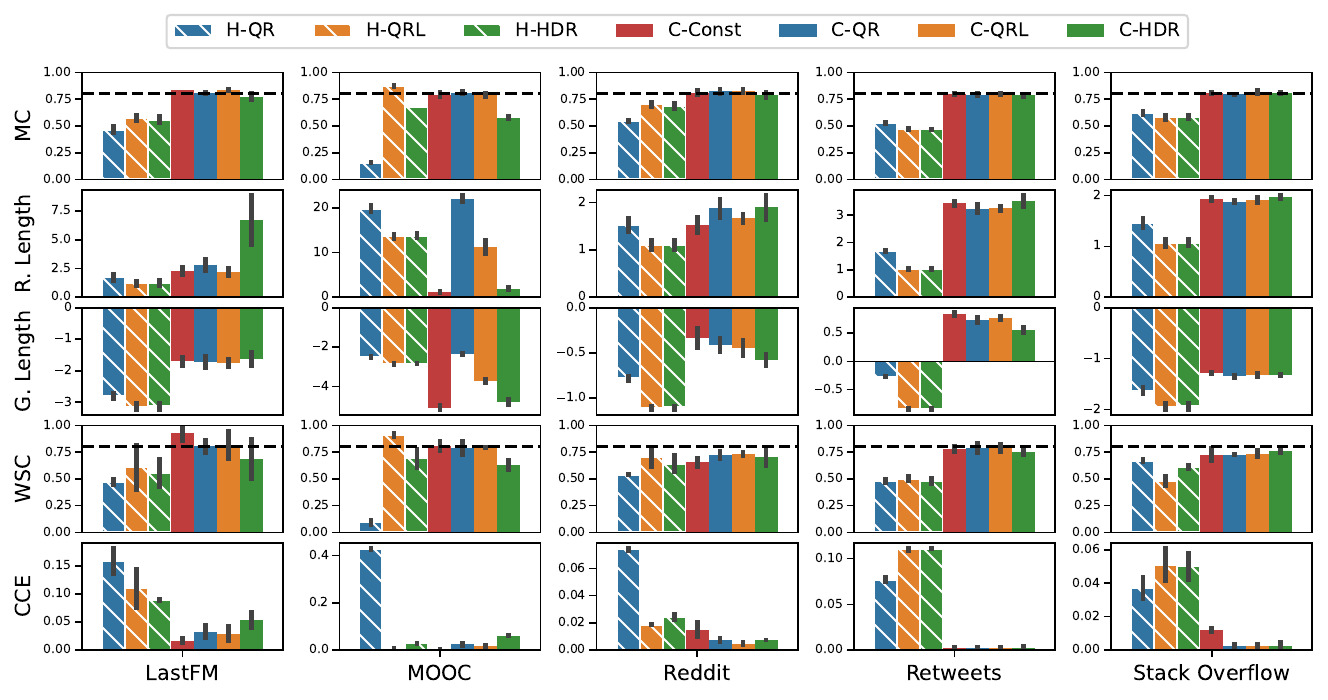}
    \caption{THP}
\end{figure}

\begin{figure}[h!]
    \centering
    \includegraphics[width=\linewidth]{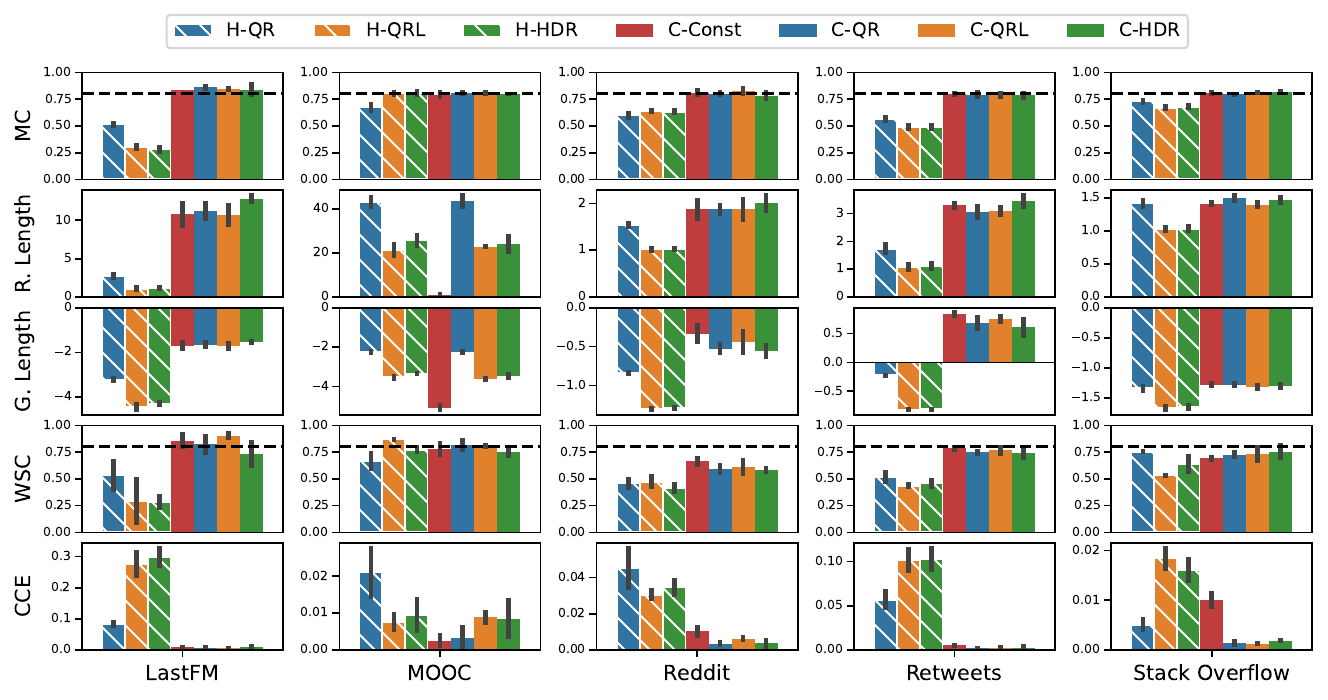}
    \caption{SAHP}
\end{figure}

\subsection{Mark}

\begin{figure}[h!]
    \centering
    \includegraphics[width=\linewidth]{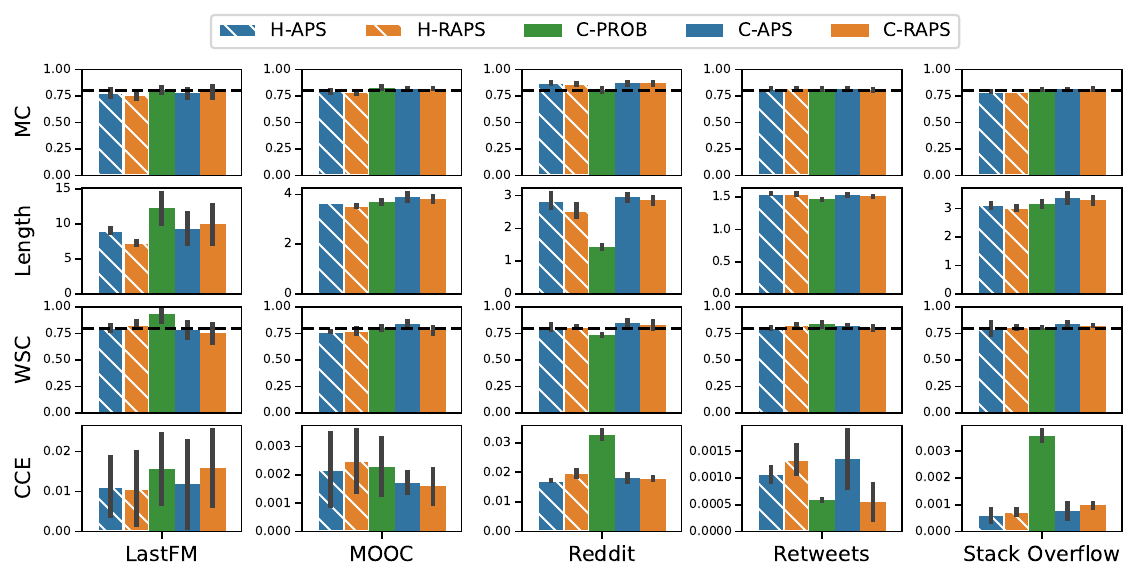}
    \caption{CLNM}
\end{figure}

\begin{figure}[h!]
    \centering
    \includegraphics[width=\linewidth]{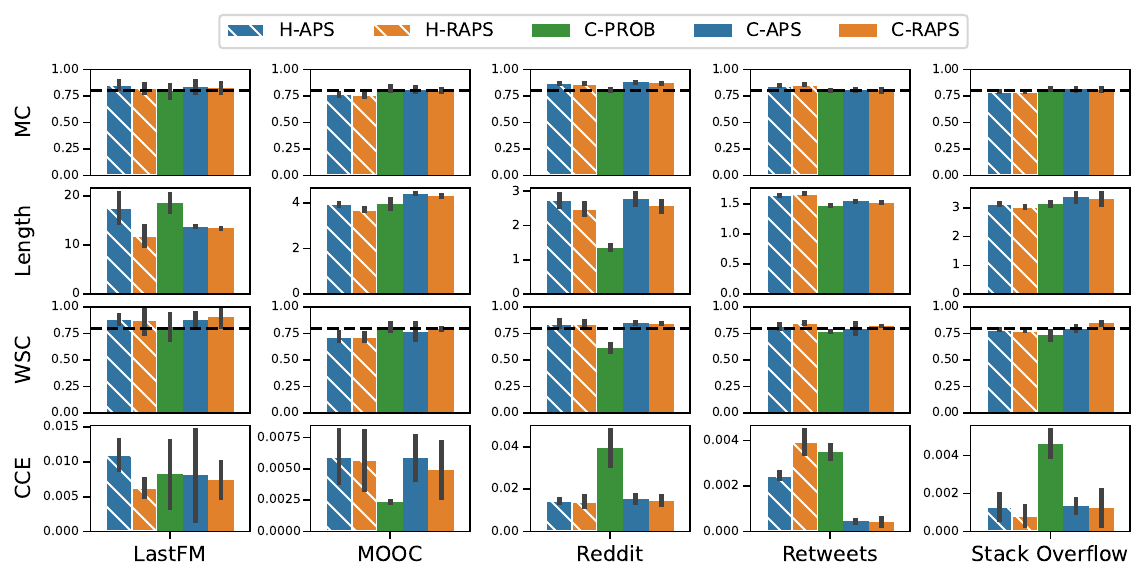}
    \caption{RMTPP}
\end{figure}

\begin{figure}[h!]
    \centering
    \includegraphics[width=\linewidth]{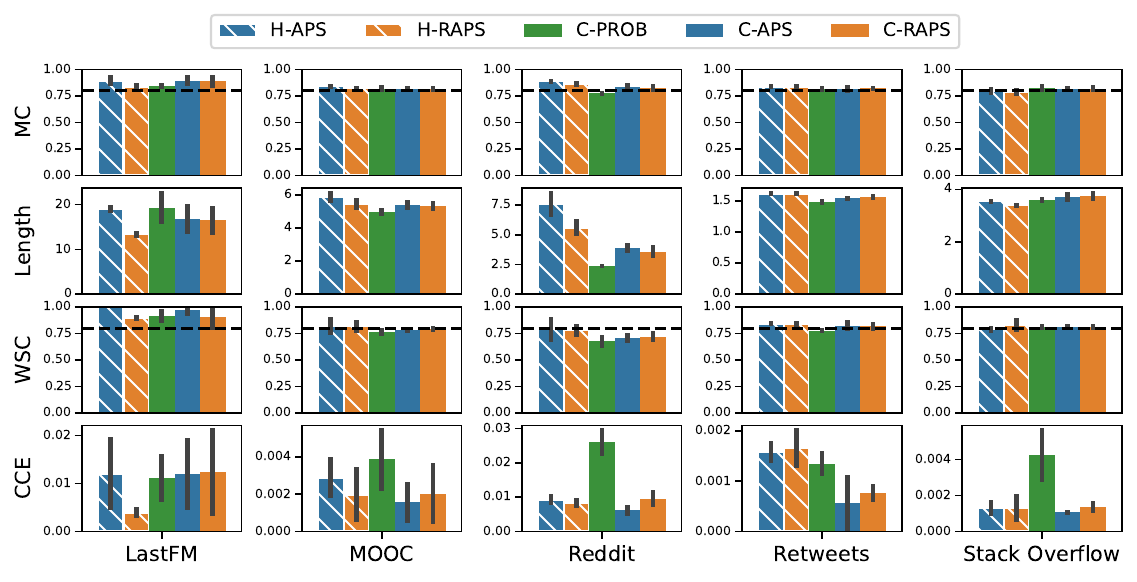}
    \caption{FNN}
\end{figure}

\begin{figure}[h!]
    \centering
    \includegraphics[width=\linewidth]{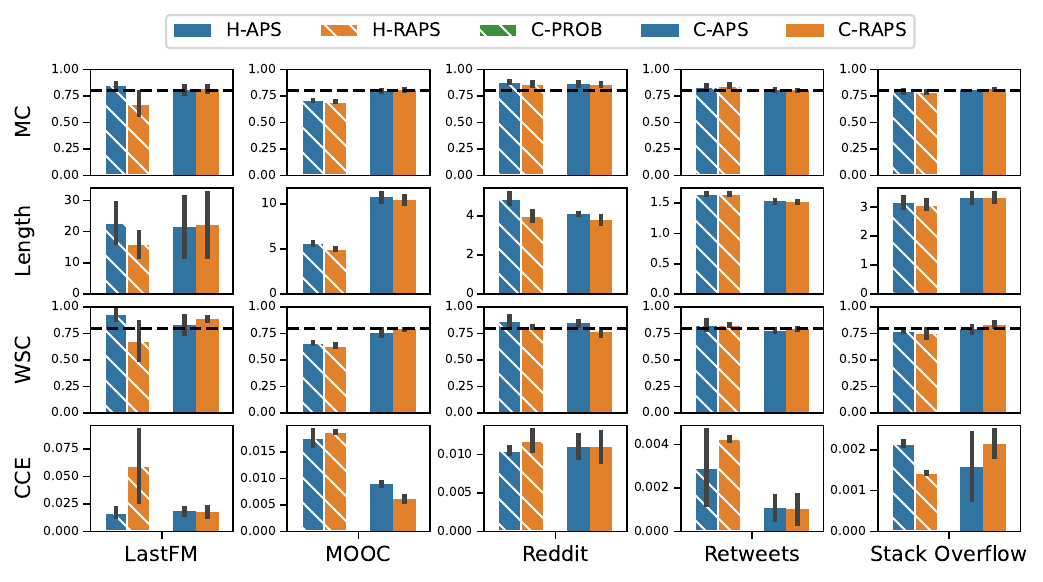}
    \caption{THP}
\end{figure}

\begin{figure}[h!]
    \centering
    \includegraphics[width=\linewidth]{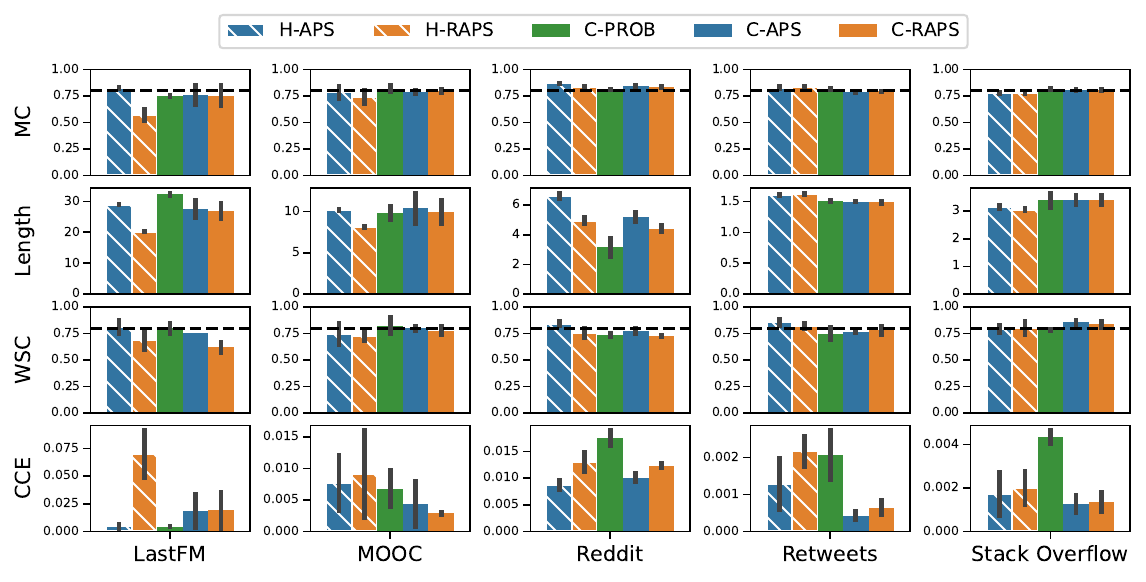}
    \caption{SAHP}
\end{figure}

\subsection{Joint}

\begin{figure}[h!]
    \centering
    \includegraphics[width=\linewidth]{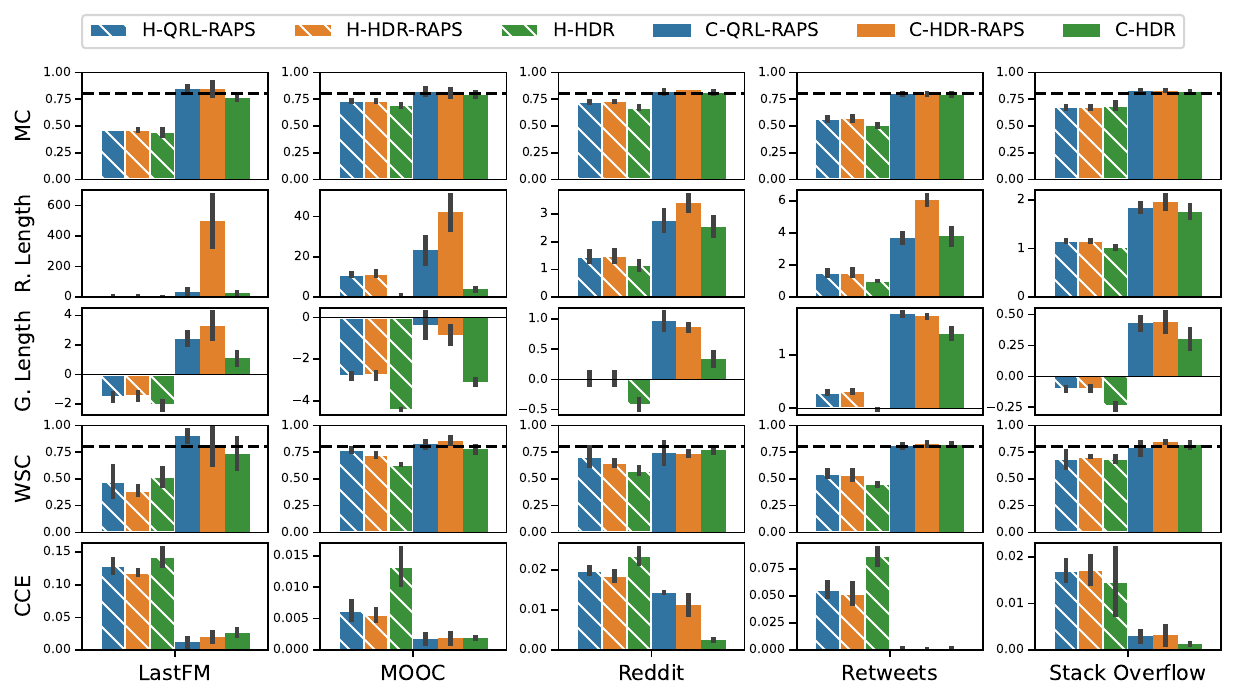}
    \caption{CLNM}
\end{figure}

\begin{figure}[h!]
    \centering
    \includegraphics[width=\linewidth]{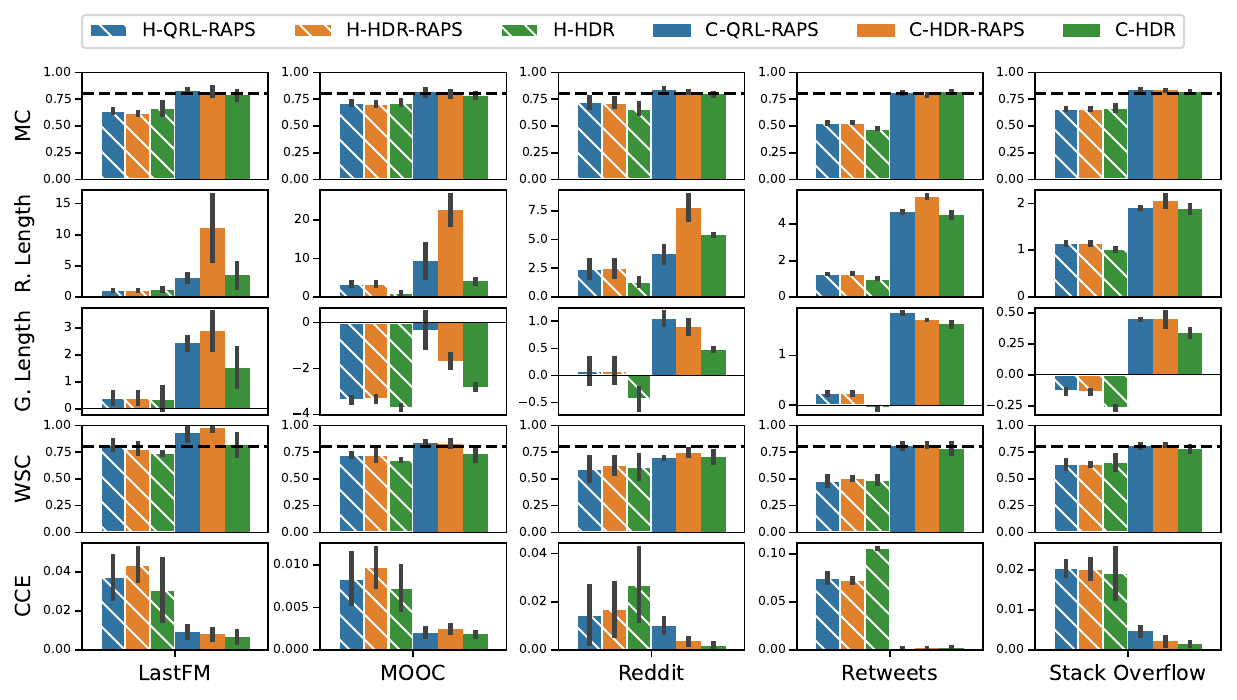}
    \caption{RMTPP}
\end{figure}

\begin{figure}[h!]
    \centering
    \includegraphics[width=\linewidth]{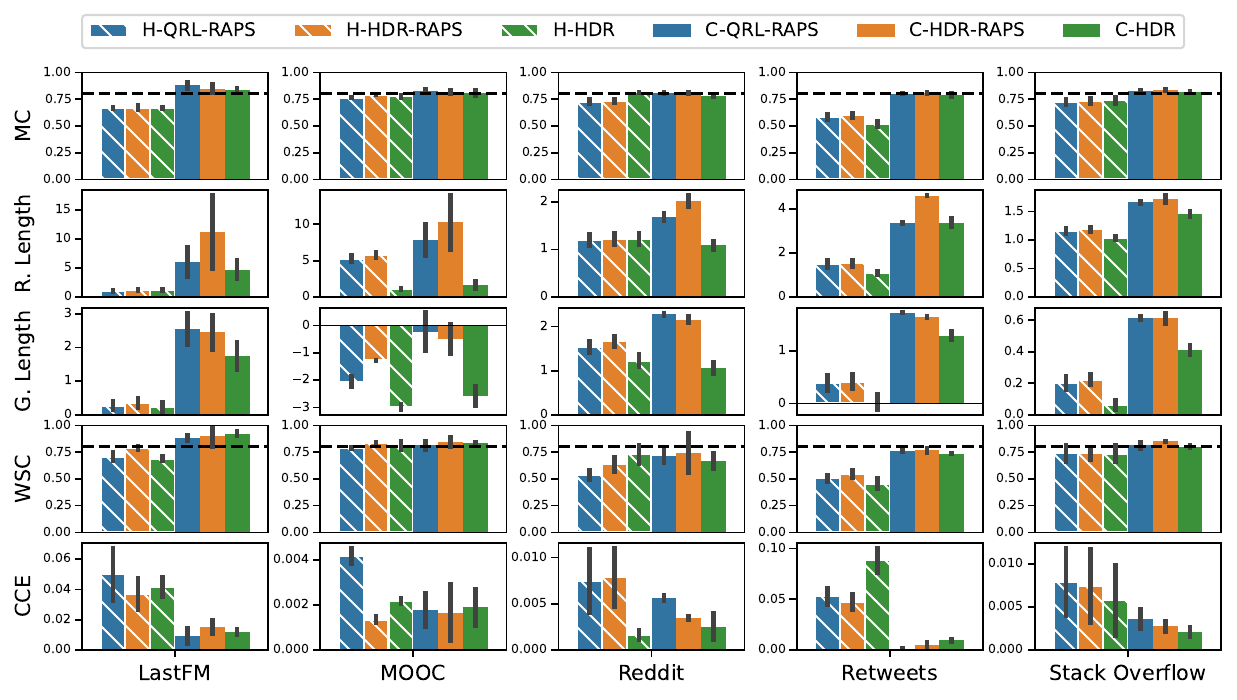}
    \caption{FNN}
\end{figure}

\begin{figure}[h!]
    \centering
    \includegraphics[width=\linewidth]{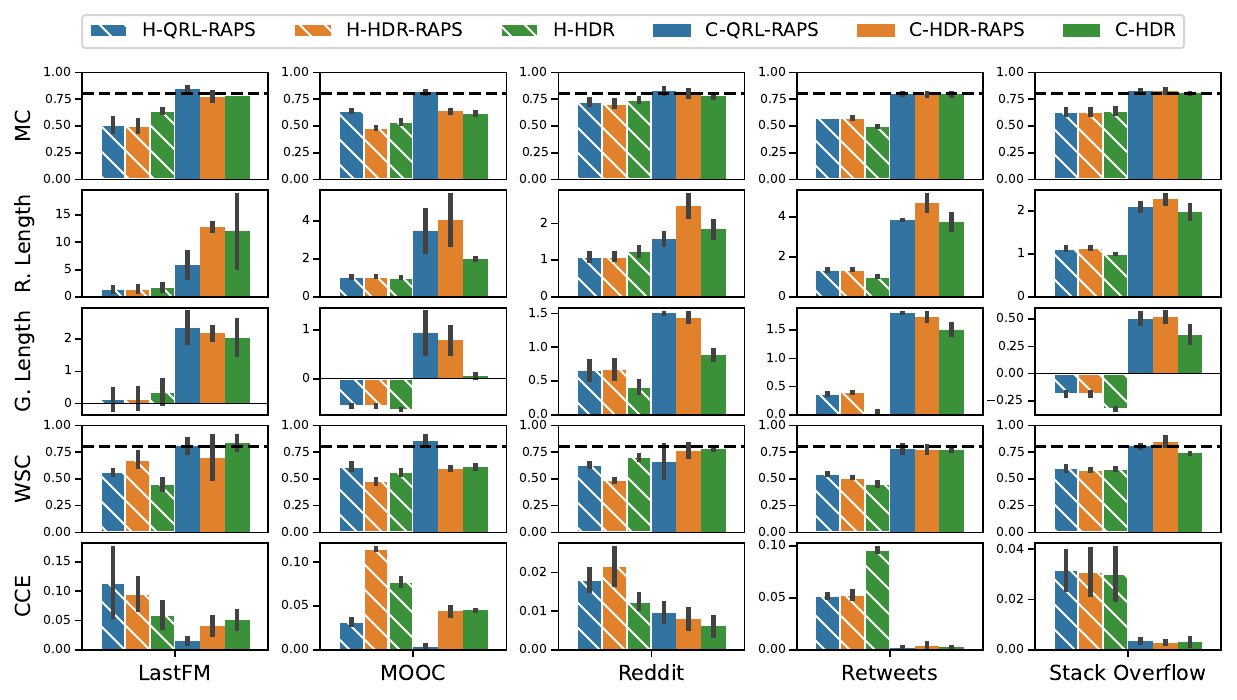}
    \caption{THP}
\end{figure}

\begin{figure}[h!]
    \centering
    \includegraphics[width=\linewidth]{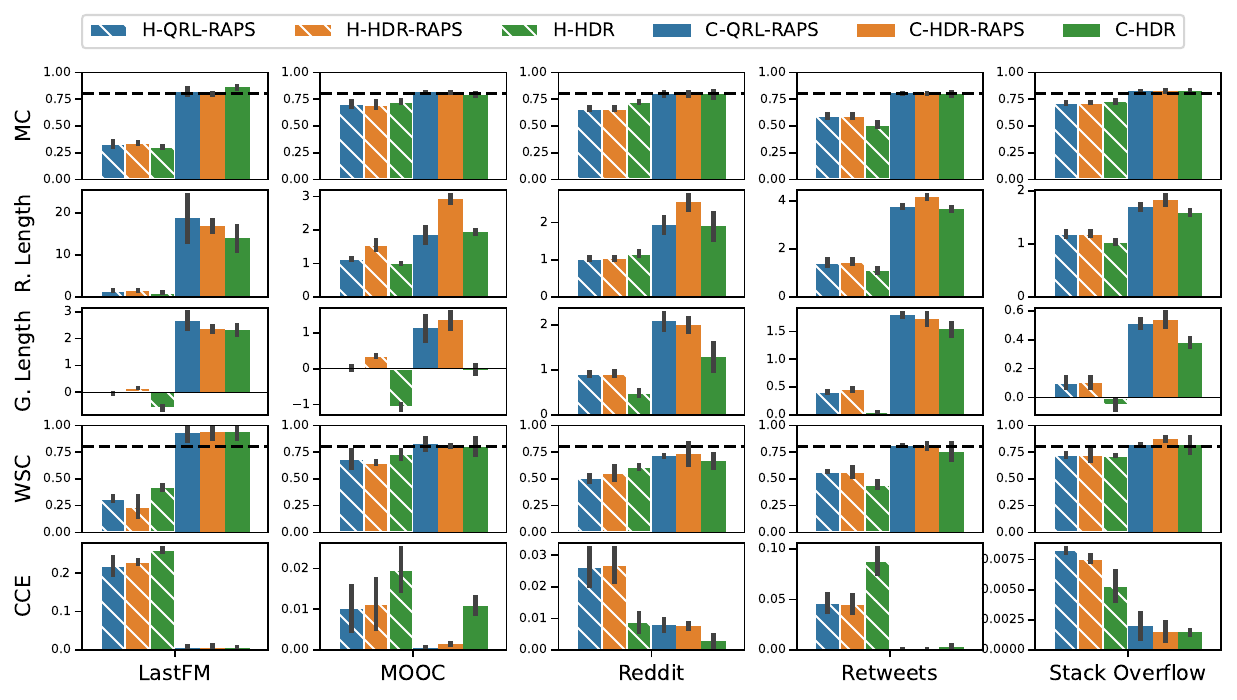}
    \caption{SAHP}
\end{figure}

\subsection{Mark conditional to time}

\begin{figure}
    \centering
    \includegraphics[width=\linewidth]{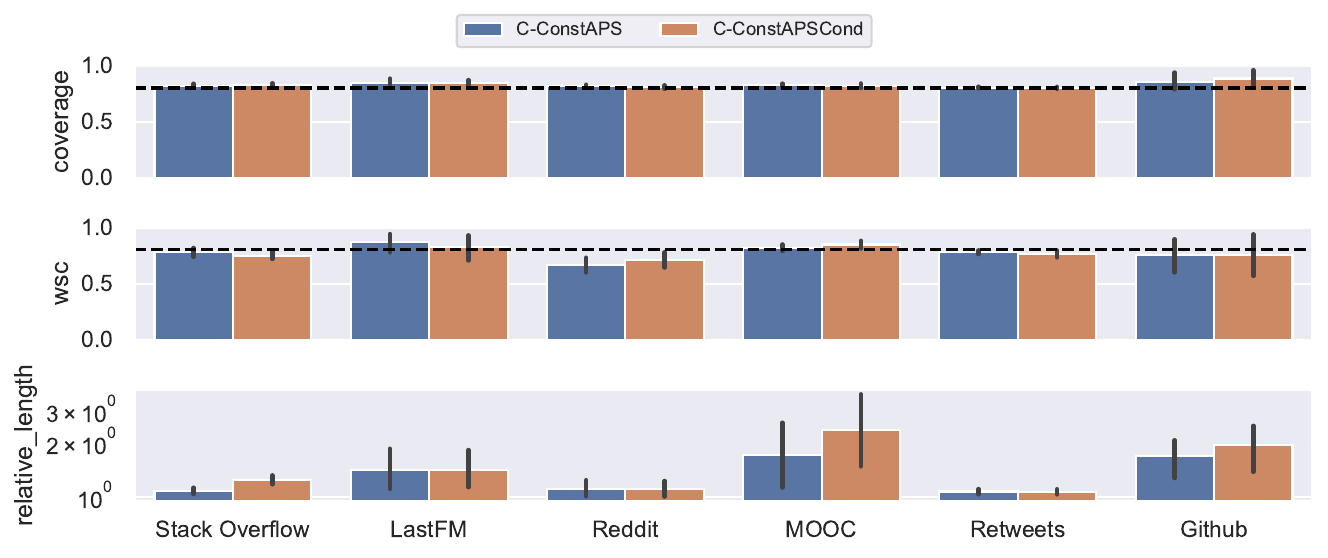}
    \caption{APS with $f(k)$ vs APS with $f(k \mid t)$ using CLNM.}
\end{figure}
